# Supplementary material for: Few-Shot Continual Learning via Flat-to-Wide Approaches
Source: arXiv:2306.14369 source file (2023-07-14)
Supplement: Supplementary file 1 [file suplementary.tex]

\documentclass[lettersize,journal]{IEEEtran}
\usepackage{amsmath,amsfonts}
% \usepackage{algorithmic}
\usepackage{algorithm}
\usepackage{array}
% \usepackage[caption=false,font=normalsize,labelfont=sf,textfont=sf]{subfig}
\usepackage{textcomp}
\usepackage{stfloats}
\usepackage{url}
\usepackage{verbatim}
\usepackage{graphicx}
% \usepackage{cite}

\usepackage{graphicx}
\usepackage{amsmath}
\usepackage{amssymb}
\usepackage{booktabs}
%\usepackage{cite}
\usepackage{amsfonts}
\usepackage{textcomp}
\usepackage{xcolor}
\usepackage{breqn}
\usepackage{multirow}
\usepackage{array}
\usepackage{threeparttable}
%\usepackage[vlined,linesnumbered,ruled]{algorithm2e}
%\usepackage{algpseudocode}
%\usepackage{algcompatible}
\usepackage{algorithm}
\usepackage{algpseudocode}
\usepackage{algorithmicx}
\usepackage{tabularx}
% \hyphenation{op-tical net-works semi-conduc-tor IEEE-Xplore}
% \def\BibTeX{{\rm B\kern-.05em{\sc i\kern-.025em b}\kern-.08em
%     T\kern-.1667em\lower.7ex\hbox{E}\kern-.125emX}}
% \hyphenation{op-tical net-works semi-conduc-tor IEEE-Xplore}
% updated with editorial comments 8/9/2021
% \addbibresource{sn-bibliography.bib}
\usepackage{balance}
\begin{document}
\onecolumn

\title{Supplementary Material for Few-Shot Continual Learning via Flat-to-Wide Approaches}
\author{Muhammad Anwar Ma'sum, Mahardhika Pratama,~\IEEEmembership{Senior member, ~IEEE}, Edwin Lughofer, Lin Liu, Habibullah, Ryszard Kowalczyk}
% \thanks{M. A. Ma’sum, M. Pratama, L. Liu, Habibullah and R. Kowalczyk are with
% STEM, University of South Australia, Adelaide, SA, 5095 Australia.
% Edwin Lughofer is with Institute for Mathematical Methods in Medicine and Databased
% Modeling, Johannes Kepler University, Altenberger Straße 69, Linz, 4040, Österreich, Austria.
% M. A. Ma’sum, and M. Pratama share equal contributions.}% <-this % stops a space
% \thanks{Manuscript received April 19, 2021; revised August 16, 2021.}
% The paper headers
\markboth{Journal of \LaTeX\ Class Files,~Vol.~14, No.~8, August~2021}%
{Shell \MakeLowercase{\textit{et al.}}: A Sample Article Using IEEEtran.cls for IEEE Journals}
% \IEEEpubid{0000--0000/00\$00.00~\copyright~2021 IEEE}
% Remember, if you use this you must call \IEEEpubidadjcol in the second
% column for its text to clear the IEEEpubid mark.
\maketitle

% \begin{abstract}
% Existing approaches on continual learning call for a lot of samples in their training processes. Such approaches are impractical for many real-world problems having limited samples because of the overfitting problem. This paper proposes a few-shot continual learning approach, termed FLat-tO-WidE AppRoach (FLOWER), where a flat-to-wide learning process finding the flat-wide minima is proposed to address the catastrophic forgetting problem. The issue of data scarcity is overcome with a data augmentation approach making use of a ball generator concept to restrict the sampling space into the smallest enclosing ball. Our numerical studies demonstrate the advantage of FLOWER achieving significantly improved performances over prior arts notably in the small base tasks. For further study, source codes of FLOWER, competitor algorithms and experimental logs are shared publicly in \url{https://github.com/anwarmaxsum/FLOWER}.
% \end{abstract}
% \begin{IEEEkeywords}
% Continual Learning, Few-Shot Learning, Incremental Learning, Lifelong Learning
% \end{IEEEkeywords}


%\bmhead{Supplementary information}

%If your article has accompanying supplementary file/s please state so here. 

%Authors reporting data from electrophoretic gels and blots should supply the full unprocessed scans for key as part of their Supplementary information. This may be requested by the editorial team/s if it is missing.

%Please refer to Journal-level guidance for any specific requirements.

% \section*{Acknowledgments}
%\bmhead{Acknowledgments}
% This work is financially supported by the University of South Australia start-up grant.

%Please refer to Journal-level guidance for any specific requirements.

% \section*{Declarations}

% %Some journals require declarations to be submitted in a standardised format. Please check the Instructions for Authors of the journal to which you are submitting to see if you need to complete this section. If yes, your manuscript must contain the following sections under the heading `Declarations':

% \begin{itemize}
% \item \textbf{Funding: }
% This work is financially supported by the University of South Australia start-up grant.
% \item \textbf{Conflict of interest: }
% The authors do not have any conflict of interest.
% \item \textbf{Ethics approval: }
% Not applicable
% \item \textbf{Consent to participate: }
% Not applicable
% \item \textbf{Consent for publication: }
% Not applicable
% \item \textbf{Availability of data and materials: }
% The datasets and the experimental result are publicly available at \url{https://github.com/anwarmaxsum/FLOWER}.
% \item \textbf{Code availability: }
% The code, simulation environment setting, and running script are publicly available at \url{https://github.com/anwarmaxsum/FLOWER}.
% \item \textbf{Authors' contributions: }
% MAM and MP designed the proposed method, conducted the data collection, developed the simulation environment, conducted experiments, evaluation, analysis, and manuscript writing. LL, EL, HH and RK contributed to the design of the proposed method, conducted method verification, analysis, provided supervision, and conducted manuscript editing.
% \end{itemize}

%\noindent
%If any of the sections are not relevant to your manuscript, please include the heading and write `Not applicable' for that section. 

%%===================================================%%
%% For presentation purpose, we have included        %%
%% \bigskip command. please ignore this.             %%
%%===================================================%%
%\bigskip
%\begin{flushleft}%
%Editorial Policies for:

%\bigskip\noindent
%Springer journals and proceedings: \url{https://www.springer.com/gp/editorial-policies}

%\bigskip\noindent
%Nature Portfolio journals: \url{https://www.nature.com/nature-research/editorial-policies}

%\bigskip\noindent
%\textit{Scientific Reports}: \url{https://www.nature.com/srep/journal-policies/editorial-policies}

%\bigskip\noindent
%BMC journals: \url{https://www.biomedcentral.com/getpublished/editorial-policies}
%\end{flushleft}
% \bibliographystyle{plain}
% \LaTeX{}
%\bibliographystyle{IEEEtran}
% argument is your BibTeX string definitions and bibliography database(s)
%\bibliography{IEEEabrv,../bib/paper}


% \section*{Declarations}
% The authors declare that they have no known competing financial interests or personal relationships that could have appeared to influence the work reported in this paper.

\begin{appendices}

\section{Proof of Theorem 1}\label{secA1}
\subsection{Lemma 2 \cite{Shi2021OvercomingCF}}
Under assumption 1 and 2, the following can be derived:
\begin{equation}\label{1}
\begin{split}
    \mathbb{E}_{z_k,\epsilon_j}[R(\Theta_{k+1})] - R(\Theta_k)\leq-\lambda_k\frac{2M-\lambda_k L(m_2+M)}{2M}||\nabla R(\Theta_k)||_{2}^{2}+\frac{\lambda_k^{2}L m_1}{2M}
\end{split}
\end{equation}
\textbf{Proof}. Assumption 1 leads to the following for all $\{\Theta,\Theta'\}\in\Re^{d}$. 
\begin{equation}\label{2}
\begin{split}
    R(\Theta)\leq R(\Theta') + \nabla R(\Theta')^{T}(\Theta-\Theta')+\frac{1}{2}L||\Theta-\Theta||_2^2
\end{split}
\end{equation}
Given the parameter update $\Theta_{k+1}=\Theta_k-\frac{\lambda_k}{M}\sum_{j=1}^{M}\nabla\mathcal{L}_{base}^{j,k}$ and $\hat{s}=\frac{1}{M}\sum_{j=1}^{M}s_{j,k}$ where $s_{j,k}=\mathcal{L}_{base}^{j,k}$, we can go further:
\begin{equation}\label{3}
    \begin{split}
        R(\Theta_{k+1})-R(\Theta_{k})\leq\nabla R(\Theta_{k})^{T}(\Theta_{k+1}-\Theta_k)+\\\frac{1}{2}L||\Theta_{k+1}-\Theta_k||_2^{2}\leq-\lambda_{k}\nabla R(\Theta_k)^{T}\hat{s}+\frac{\lambda_{k}^{2}L}{2}||\hat{s}||_{2}^{2} 
    \end{split}
\end{equation}
Recall that $\mathbb{E}_{z_k,\epsilon_j}[.]$ denotes the expectation w.r.t the joint distribution of random variables $z_k,\epsilon_j$ which can be applied on both sides of \eqref{3}.
\begin{equation}\label{4}
    \begin{split}
        \mathbb{E}_{z_k,\epsilon_j}[R(\Theta_{k+1})]-R(\Theta_k)\leq-\lambda_k\nabla R(\Theta_k)^{T}\mathbb{E}_{z_k,\epsilon_j}[\hat{s}]+\frac{\lambda_{k}^{2}L}{2}\mathbb{E}_{z_k,\epsilon_j}[||\hat{s}||_2^{2}]
    \end{split}
\end{equation}
Because of the second condition of assumption 2 and the fact that $\Theta_{k+1}$ is a factor of $z_k,\epsilon_j$, $\mathbb{E}_{z_k,\epsilon_j}[\hat{s}]$ meets the following condition. 
\begin{equation}\label{5}
    \mathbb{E}_{z_k,\epsilon_j}[\hat{s}]=\frac{1}{M}\sum_{j=1}^{M}\mathbb{E}_{z_k,\epsilon_j}[s_{j,k}]=\nabla R(\Theta_k)
\end{equation}
Suppose $\epsilon_j$ is sampled without replacement from $P(\epsilon)$, following \cite{Kullback1962MathematicalSJ} and the condition 3 of assumption 2, we can obtain:
\begin{equation}\label{6}
    \mathbb{V}_{z_k,\epsilon_j}[\hat{s}]\leq\frac{\mathbb{V}_{z_k,\epsilon_j} s_{j,k}}{M}\leq\frac{m_1}{M}+\frac{m_2}{M}||\nabla R(\Theta_k)||_{2}^{2}
\end{equation}
Combining \eqref{5} and \eqref{6}, we find:
\begin{equation}\label{7}
\begin{split}
    \mathbb{E}_{z_k,\epsilon_j}[||\hat{s}||_2^2]=\mathbb{V}_{z_k,\epsilon_j}[\hat{b}]+||\mathbb{E}_{z_k,\epsilon_j}[\hat{s}]||_{2}^{2}\leq\frac{m_1}{M}+\frac{m_2+M}{M}||\nabla R(\Theta_k)||_2^{2}
    \end{split}
\end{equation}
The proof is completed by combining \eqref{4},\eqref{5},\eqref{7}. 

\subsection{Lemma 3 \cite{Shi2021OvercomingCF}}
Because of assumptions 1-3, the following lemma is derived.
\begin{equation}\label{8}
    \liminf_{k\rightarrow\infty}{\mathbb{E}[||\nabla R(\Theta_k)||_{2}^{2}]}=0
\end{equation}
\textbf{Proof}. Note that $\lim_{k\rightarrow\infty}\lambda_k=0$ as per assumption 3 leading to $k\in\mathbb{N},\lambda_k L(m_2+M)\leq M$ without loss of generalization. Suppose that $\mathbb{E}[.]$ stands for the total expectations across all random variables $z_k,\epsilon_j$, we can express $\mathbb{E}[R(\Theta_k)]$:
\begin{equation}\label{9}
    \mathbb{E}[R(\Theta_k)]=\mathbb{E}_{z_0,\epsilon_0}\mathbb{E}_{z_1,\epsilon_1}...\mathbb{E}_{z_{k-1},\epsilon_{k-1}}[R(\Theta_k)]
\end{equation}
Applying the total expectation to \eqref{1}, we observe:
\begin{equation}\label{10}
\begin{split}
    \mathbb{E}[R(\Theta_{k+1})]-\mathbb{E}[R(\Theta_k)]\leq-\frac{\lambda_k}{2}\mathbb{E}[||\nabla R(\Theta_k)||_2^2]+\frac{\lambda_k^2 L m_1}{2M}
\end{split}    
\end{equation}
For $k=[0,K]$, summation is applied to both sides of \eqref{10}:
\begin{equation}\label{11}
    \begin{split}
    R^*-\mathbb{E}[R(\Theta_1)]\leq\mathbb{E}[R(\Theta_{K+1})]-\mathbb{E}[R(\Theta_0)]\leq\frac{-1}{2}\sum_{k=0}^{K}\lambda_l\mathbb{E}[||\nabla R(\Theta_k)||_2^2]+\frac{Lm_1}{2M}\sum_{k=0}^{K}\lambda_k^2
    \end{split}
\end{equation}
where $R^*$ is the lower bound of condition 1 of assumption 2. we further derive \eqref{11}:
\begin{equation}\label{12}
\begin{split}
    \sum_{k=0}^{K}\lambda_k\mathbb{E}[||\nabla R(\Theta)||_{2}^{2}]\leq 2(\mathbb{E}[R(\Theta_1)]-R^*)+\frac{L m_1}{M}\sum_{k=0}^{K}\lambda_k^2
    \end{split}
\end{equation}
Using the second condition of assumption 3, we obtain:
\begin{equation}\label{13}
    \begin{split}
    \lim_{K\rightarrow\infty}\mathbb{E}[\sum_{k=0}^{K}\lambda_k||\nabla R(\Theta_k)||_2^2]\leq 2(\mathbb{E}[R(\Theta_0)]-R^*)+\lim_{k\rightarrow\infty}\frac{L m_1}{M}\sum_{k=0}^{K}\lambda_{k}^2<\infty    
    \end{split}
\end{equation}
We divide both sides \eqref{12} by $\sum_{k=1}^{K}\lambda_k$ and use assumption 3:
\begin{equation}\label{14}
    \lim_{K\rightarrow\infty}\mathbb{E}[\frac{\sum_{k=1}^{K}\lambda_{k}||\nabla R(\Theta_k)||_2^2}{\sum_{k=1}^{K}\lambda_2}]=0
\end{equation}
\eqref{14} is a weighted average operation with $\lambda_k$ as a weight. As a result, $||\nabla R(\Theta_k)||_2^2$ must asymptotically approach zero, thus proving \eqref{8}. 
\subsection{Proof of Theorem 1 \cite{Shi2021OvercomingCF}}
Recall that because of assumptions 1-3 and that the risk function $R$ is twice differentiable and as a result of assumption 1 $||\nabla R(\Theta)||_2^2$ is $L_{2}$-smooth with $L_2>0$, the following holds. 
\begin{equation}\label{15}
    \lim_{k\rightarrow\infty}\mathbb{E}[||\nabla R(\Theta_k)||_2^2] = 0
\end{equation}
\textbf{Proof}. Let $Q(\Theta)=||R(\Theta)||_2^2$, we observe:
\begin{equation}\label{16}
    \begin{split}
    \mathbb{E}_{z_k,\epsilon_j}[Q(\Theta_{k+1})] - Q(\Theta_k)\leq\nabla Q(\Theta_k)^{T}\mathbb{E}_{z_k,\epsilon_j}[(\Theta_{k+1}-\Theta_k)]\\+\frac{1}{2}L_2\mathbb{E}_{z_k,\epsilon_j}[||\Theta_{k+1}-\Theta_k||_2^2]\\\leq-\lambda_k\nabla Q(\Theta_k)^{T}\mathbb{E}_{z_k,\epsilon_j}[\hat{s}]+\frac{\lambda_k^2L_2}{2}\mathbb{E}_{z_k,\epsilon_k}[||\hat{s}||_2^2]\\\leq-2\lambda_k\nabla R(\Theta_k)^{T}\nabla^2R(\Theta_k)\mathbb{E}_{z_k,\epsilon_j}[\hat{g}]+\frac{\lambda_k^2L_2}{2}\mathbb{E}_{z_k,\epsilon_j}[||\hat{s}||_2^2]\\\leq2\lambda_kL||\nabla R(\Theta_k)||_2^2||\nabla^2R(\Theta_k)||_2||\mathbb{E}_{z_k,\epsilon_j}||_2+\frac{\lambda_k^2L_2}{2}\mathbb{E}_{z_k,\epsilon_j}[||\hat{g}||_2^2]\\\leq 2\lambda_k L||\nabla R(\Theta_k)||_2^2+\frac{\lambda_k^2L_2}{2}(\frac{m1}{M}+\frac{m_2+M}{M}||\nabla R(\Theta_k)||_2^2)
    \end{split}
\end{equation}
Using the total expectations to both sides of \eqref{16} leads to
\begin{equation}\label{17}
    \begin{split}
        \mathbb{E}[Q(\Theta_{k+1})]-\mathbb{E}[F(\Theta_k)]\leq2\lambda_2L\mathbb{E}[||\nabla R(\Theta_k)||_2^2]+\frac{\lambda_k^2L_2}{2}(\frac{m_1}{M}+\frac{m_2+M}{M}\mathbb{E}[||\nabla R(\Theta_k)||_2^2])
    \end{split}
\end{equation}
$2\lambda_kL\mathbb{E}[||\nabla R(\Theta_k)||_2^]$ is the term of a convergent sum as per \eqref{13} as well as that $\frac{\lambda_k^2L_2}{2}(\frac{m_1}{M}+\frac{m_2+M}{M}\mathbb{E}[||\nabla R(\Theta_k)||_2^2])$ because of the convergence of $\sum_{k=1}^{\infty}\lambda_k^2$. Therefore, the upper bound of \eqref{17} implies a convergent sum. We define:
\begin{equation}\label{18}
    A_{K}^{+}=\sum_{k=0}^{K-1}\max{(0,\mathbb{E}[Q(\Theta_{k+1})]-\mathbb{E}[Q(\Theta_k)])}
\end{equation}
\begin{equation}\label{18}
    A_{K}^{-}=\sum_{k=0}^{K-1}\max{(0,\mathbb{E}[Q(\Theta_{k})]-\mathbb{E}[Q(\Theta_{k+1})])}
\end{equation}
As per \eqref{17}, the bound of $\mathbb{E}[Q(\Theta_{k+1})]-\mathbb{E}[Q(\Theta_k)]$ are positive and the term of convergent sum. $A_{K}^{+}$ and $A_{K}^{-}$ converge as the sum of the bound of $\mathbb{E}[Q(\Theta_{K+1})]-\mathbb{E}[Q(\Theta_k)]$. $Q(\Theta_K)$ also converges due to $Q(\Theta_K)=Q(\Theta_0)+A_{K}^{+}-A_{K}^{-}$ for $K\in\mathbb{N}$. We can then prove the theorem 1 also justified by Lemma 3.
%\end{appendices}


\section{Complete Numerical Results of 5-Shot Experiments}  

\begin{table*}
% \footnotesize
\small
\centering
% \begin{tabularx}{1.0\textwidth}{lXXXXXXXXX\fontsize{3}{5}r}
% \begin{tabularx}{1.0\textwidth}{lXXXXXXXXXr}
% \begin{tabular}{1.0\textwidth}{lcccccccccc}
% \begin{tabular}{lcccccccccc}
\begin{tabular}{lccccccccccccc}
\hline
\cline{1-11}
{}                                                           & \multicolumn{9}{c}{{\textbf{Session}}}         & {}                                                      \\ \cline{2-10}
\multirow{-2}{*}{{\textbf{Method}}} & \centering{1}              & \centering{2}              & \centering{3}              & \centering{4}              & \centering{5}              & \centering{6}              & \centering{7}              & \centering{8}              & \centering{9}              & \multirow{-2}{*}{{\textbf{Avg}}} \\ \cline{1-11} \hline 
\multicolumn{11}{c}{{\textbf{Base classes = 60}}} \\ \hline
{Baseline \cite{Shi2021OvercomingCF}}                          & {\begin{tabular}[c]{@{}l@{}}66.78\\ $\pm$0.00\end{tabular}}          & {\begin{tabular}[c]{@{}l@{}}61.29\\ $\pm$0.13\end{tabular}}          & {\begin{tabular}[c]{@{}l@{}}57.25\\ $\pm$0.21\end{tabular}}          & {\begin{tabular}[c]{@{}l@{}}54.17\\ $\pm$0.16\end{tabular}}          & {\begin{tabular}[c]{@{}l@{}}51.54\\ $\pm$0.17\end{tabular}}          & {\begin{tabular}[c]{@{}l@{}}49.00\\ $\pm$0.28\end{tabular}}          & {\begin{tabular}[c]{@{}l@{}}46.56\\ $\pm$0.25\end{tabular}}          & {\begin{tabular}[c]{@{}l@{}}44.99\\ $\pm$0.27\end{tabular}}          & {\begin{tabular}[c]{@{}l@{}}43.78\\ $\pm$0.34\end{tabular}}          & {\begin{tabular}[c]{@{}l@{}}52.82\\ $\pm$0.20\end{tabular}}          \\ \hline
{F2M \cite{Shi2021OvercomingCF}}                               & {\begin{tabular}[c]{@{}l@{}}66.07\\ $\pm$0.00\end{tabular}}          & {\begin{tabular}[c]{@{}l@{}}61.05\\ $\pm$0.12\end{tabular}}          & {\begin{tabular}[c]{@{}l@{}}56.82\\ $\pm$0.23\end{tabular}}          & {\begin{tabular}[c]{@{}l@{}}53.51\\ $\pm$0.28\end{tabular}}          & {\begin{tabular}[c]{@{}l@{}}50.76\\ $\pm$0.32\end{tabular}}          & {\begin{tabular}[c]{@{}l@{}}48.26\\ $\pm$0.34\end{tabular}}          & {\begin{tabular}[c]{@{}l@{}}45.79\\ $\pm$0.29\end{tabular}}          & {\begin{tabular}[c]{@{}l@{}}44.07\\ $\pm$0.26\end{tabular}}          & {\begin{tabular}[c]{@{}l@{}}42.62\\ $\pm$0.19\end{tabular}}          & {\begin{tabular}[c]{@{}l@{}}52.11\\ $\pm$0.23\end{tabular}}          \\ \hline
{FSLL\cite{Mazumder2021FewShotLL}}                              & {\begin{tabular}[c]{@{}l@{}}66.98\\ $\pm$0.00\end{tabular}}          & {\begin{tabular}[c]{@{}l@{}}57.23\\ $\pm$0.39\end{tabular}}          & {\begin{tabular}[c]{@{}l@{}}52.47\\ $\pm$0.34\end{tabular}}          & {\begin{tabular}[c]{@{}l@{}}49.66\\ $\pm$0.42\end{tabular}}          & {\begin{tabular}[c]{@{}l@{}}47.45\\ $\pm$0.46\end{tabular}}          & {\begin{tabular}[c]{@{}l@{}}45.2\\ $\pm$0.38\end{tabular}}           & {\begin{tabular}[c]{@{}l@{}}43.29\\ $\pm$0.42\end{tabular}}          & {\begin{tabular}[c]{@{}l@{}}42.06\\ $\pm$0.47\end{tabular}}          & {\begin{tabular}[c]{@{}l@{}}41.18\\ $\pm$0.42\end{tabular}}          & {\begin{tabular}[c]{@{}l@{}}49.50\\ $\pm$0.37\end{tabular}}          \\ \hline
{ICARL\cite{Rebuffi2017iCaRLIC}}                             & {\begin{tabular}[c]{@{}l@{}}66.05\\ $\pm$0.00\end{tabular}}          & {\begin{tabular}[c]{@{}l@{}}56.47\\ $\pm$0.18\end{tabular}}          & {\begin{tabular}[c]{@{}l@{}}53.26\\ $\pm$0.3\end{tabular}}           & {\begin{tabular}[c]{@{}l@{}}50.14\\ $\pm$0.11\end{tabular}}          & {\begin{tabular}[c]{@{}l@{}}47.55\\ $\pm$0.10\end{tabular}}          & {\begin{tabular}[c]{@{}l@{}}45.08\\ $\pm$0.24\end{tabular}}          & {\begin{tabular}[c]{@{}l@{}}42.47\\ $\pm$0.34\end{tabular}}          & {\begin{tabular}[c]{@{}l@{}}41.04\\ $\pm$0.39\end{tabular}}          & {\begin{tabular}[c]{@{}l@{}}39.60\\ $\pm$0.22\end{tabular}}          & {\begin{tabular}[c]{@{}l@{}}49.07\\ $\pm$0.21\end{tabular}}          \\ \hline
{Rebalance\cite{Hou2019LearningAU}}                         & {\begin{tabular}[c]{@{}l@{}}66.45\\ $\pm$0.00\end{tabular}}          & {\begin{tabular}[c]{@{}l@{}}60.66\\ $\pm$0.21\end{tabular}}          & {\begin{tabular}[c]{@{}l@{}}55.61\\ $\pm$0.18\end{tabular}}          & {\begin{tabular}[c]{@{}l@{}}51.38\\ $\pm$0.12\end{tabular}}          & {\begin{tabular}[c]{@{}l@{}}47.93\\ $\pm$0.25\end{tabular}}          & {\begin{tabular}[c]{@{}l@{}}44.64\\ $\pm$0.25\end{tabular}}          & {\begin{tabular}[c]{@{}l@{}}41.40\\ $\pm$0.18\end{tabular}}          & {\begin{tabular}[c]{@{}l@{}}38.75\\ $\pm$0.41\end{tabular}}          & {\begin{tabular}[c]{@{}l@{}}37.11\\ $\pm$0.39\end{tabular}}          & {\begin{tabular}[c]{@{}l@{}}49.33\\ $\pm$0.22\end{tabular}}          \\ \hline
{ICARL+\cite{Rebuffi2017iCaRLIC}}                            & {\begin{tabular}[c]{@{}l@{}}61.31\\ $\pm$0.30\end{tabular}}          & {\begin{tabular}[c]{@{}l@{}}46.32\\ $\pm$0.85\end{tabular}}          & {\begin{tabular}[c]{@{}l@{}}42.94\\ $\pm$1.57\end{tabular}}          & {\begin{tabular}[c]{@{}l@{}}37.63\\ $\pm$1.44\end{tabular}}          & {\begin{tabular}[c]{@{}l@{}}30.49\\ $\pm$1.36\end{tabular}}          & {\begin{tabular}[c]{@{}l@{}}24.00\\ $\pm$1.53\end{tabular}}          & {\begin{tabular}[c]{@{}l@{}}20.89\\ $\pm$1.66\end{tabular}}          & {\begin{tabular}[c]{@{}l@{}}18.80\\ $\pm$1.69\end{tabular}}          & {\begin{tabular}[c]{@{}l@{}}17.21\\ $\pm$1.49\end{tabular}}          & {\begin{tabular}[c]{@{}l@{}}33.29\\ $\pm$1.32\end{tabular}}          \\ \hline
{EEIL+\cite{Castro2018EndtoEndIL}}                             & {\begin{tabular}[c]{@{}l@{}}61.31\\ $\pm$0.30\end{tabular}}          & {\begin{tabular}[c]{@{}l@{}}46.58\\ $\pm$0.86\end{tabular}}          & {\begin{tabular}[c]{@{}l@{}}44.00\\ $\pm$1.53\end{tabular}}          & {\begin{tabular}[c]{@{}l@{}}37.29\\ $\pm$1.35\end{tabular}}          & {\begin{tabular}[c]{@{}l@{}}33.14\\ $\pm$1.20\end{tabular}}          & {\begin{tabular}[c]{@{}l@{}}27.12\\ $\pm$1.47\end{tabular}}          & {\begin{tabular}[c]{@{}l@{}}24.10\\ $\pm$1.54\end{tabular}}          & {\begin{tabular}[c]{@{}l@{}}21.57\\ $\pm$1.75\end{tabular}}          & {\begin{tabular}[c]{@{}l@{}}19.58\\ $\pm$1.26\end{tabular}}          & {\begin{tabular}[c]{@{}l@{}}34.97\\ $\pm$1.25\end{tabular}}          \\ \hline
{Rebalance+\cite{Hou2019LearningAU}}                        & {\begin{tabular}[c]{@{}l@{}}61.31\\ $\pm$0.30\end{tabular}}          & {\begin{tabular}[c]{@{}l@{}}47.80\\ $\pm$0.77\end{tabular}}          & {\begin{tabular}[c]{@{}l@{}}39.31\\ $\pm$1.58\end{tabular}}          & {\begin{tabular}[c]{@{}l@{}}31.91\\ $\pm$1.37\end{tabular}}          & {\begin{tabular}[c]{@{}l@{}}25.68\\ $\pm$1.28\end{tabular}}          & {\begin{tabular}[c]{@{}l@{}}21.35\\ $\pm$1.43\end{tabular}}          & {\begin{tabular}[c]{@{}l@{}}18.67\\ $\pm$1.50\end{tabular}}          & {\begin{tabular}[c]{@{}l@{}}17.24\\ $\pm$1.52\end{tabular}}          & {\begin{tabular}[c]{@{}l@{}}14.17\\ $\pm$1.37\end{tabular}}          & {\begin{tabular}[c]{@{}l@{}}30.83\\ $\pm$1.24\end{tabular}}          \\ \hline
{TOPIC+\cite{Tao2020FewShotCL}}                            & {\begin{tabular}[c]{@{}l@{}}61.31\\ $\pm$0.30\end{tabular}}          & {\begin{tabular}[c]{@{}l@{}}50.09\\ $\pm$0.70\end{tabular}}          & {\begin{tabular}[c]{@{}l@{}}45.17\\ $\pm$1.04\end{tabular}}          & {\begin{tabular}[c]{@{}l@{}}41.16\\ $\pm$1.02\end{tabular}}          & {\begin{tabular}[c]{@{}l@{}}37.48\\ $\pm$0.83\end{tabular}}          & {\begin{tabular}[c]{@{}l@{}}35.52\\ $\pm$1.17\end{tabular}}          & {\begin{tabular}[c]{@{}l@{}}32.19\\ $\pm$1.10\end{tabular}}          & {\begin{tabular}[c]{@{}l@{}}29.46\\ $\pm$1.13\end{tabular}}          & {\begin{tabular}[c]{@{}l@{}}24.42\\ $\pm$0.96\end{tabular}}          & {\begin{tabular}[c]{@{}l@{}}39.64\\ $\pm$0.92\end{tabular}}          \\ \hline
{\textbf{FLOWER}}                   & {\textbf{\begin{tabular}[c]{@{}l@{}}68.83\\ $\pm$0.00\end{tabular}}} & {\textbf{\begin{tabular}[c]{@{}l@{}}63.27\\ $\pm$0.09\end{tabular}}} & {\textbf{\begin{tabular}[c]{@{}l@{}}59.00\\ $\pm$0.16\end{tabular}}} & {\textbf{\begin{tabular}[c]{@{}l@{}}55.61\\ $\pm$0.18\end{tabular}}} & {\textbf{\begin{tabular}[c]{@{}l@{}}52.64\\ $\pm$0.22\end{tabular}}} & {\textbf{\begin{tabular}[c]{@{}l@{}}49.96\\ $\pm$0.20\end{tabular}}} & {\textbf{\begin{tabular}[c]{@{}l@{}}47.56\\ $\pm$0.18\end{tabular}}} & {\textbf{\begin{tabular}[c]{@{}l@{}}45.86\\ $\pm$0.16\end{tabular}}} & {\textbf{\begin{tabular}[c]{@{}l@{}}44.40\\ $\pm$0.21\end{tabular}}} & {\textbf{\begin{tabular}[c]{@{}l@{}}54.13\\ $\pm$0.16\end{tabular}}} \\ \hline
\multicolumn{11}{c}{{\textbf{Base classes = 20}}} \\ \hline
{Baseline\cite{Shi2021OvercomingCF}}                          & {\begin{tabular}[c]{@{}l@{}}67.90\\ $\pm$0.00\end{tabular}}          & {\begin{tabular}[c]{@{}l@{}}46.32\\ $\pm$0.40\end{tabular}}          & {\begin{tabular}[c]{@{}l@{}}37.24\\ $\pm$0.6\end{tabular}}           & {\begin{tabular}[c]{@{}l@{}}30.13\\ $\pm$0.44\end{tabular}}          & {\begin{tabular}[c]{@{}l@{}}25.56\\ $\pm$0.28\end{tabular}}          & {\begin{tabular}[c]{@{}l@{}}22.11\\ $\pm$0.34\end{tabular}}          & {\begin{tabular}[c]{@{}l@{}}20.03\\ $\pm$0.40\end{tabular}}          & {\begin{tabular}[c]{@{}l@{}}18.14\\ $\pm$0.31\end{tabular}}          & {\begin{tabular}[c]{@{}l@{}}16.80\\ $\pm$0.32\end{tabular}}          & {\begin{tabular}[c]{@{}l@{}}31.58\\ $\pm$0.34\end{tabular}}          \\ \hline
{F2M\cite{Shi2021OvercomingCF}}                               & {\begin{tabular}[c]{@{}l@{}}65.45\\ $\pm$0.00\end{tabular}}          & {\begin{tabular}[c]{@{}l@{}}45.70\\ $\pm$0.55\end{tabular}}          & {\begin{tabular}[c]{@{}l@{}}36.15\\ $\pm$0.34\end{tabular}}          & {\begin{tabular}[c]{@{}l@{}}29.19\\ $\pm$0.20\end{tabular}}          & {\begin{tabular}[c]{@{}l@{}}24.73\\ $\pm$0.19\end{tabular}}          & {\begin{tabular}[c]{@{}l@{}}21.29\\ $\pm$0.23\end{tabular}}          & {\begin{tabular}[c]{@{}l@{}}19.18\\ $\pm$0.25\end{tabular}}          & {\begin{tabular}[c]{@{}l@{}}17.18\\ $\pm$0.12\end{tabular}}          & {\begin{tabular}[c]{@{}l@{}}15.91\\ $\pm$0.12\end{tabular}}          & {\begin{tabular}[c]{@{}l@{}}30.53\\ $\pm$0.22\end{tabular}}          \\ \hline
{FSLL\cite{Mazumder2021FewShotLL}}                              & {\begin{tabular}[c]{@{}l@{}}68.05\\ $\pm$0.00\end{tabular}}          & {\begin{tabular}[c]{@{}l@{}}47.05\\ $\pm$0.33\end{tabular}}          & {\begin{tabular}[c]{@{}l@{}}37.74\\ $\pm$0.52\end{tabular}}          & {\begin{tabular}[c]{@{}l@{}}30.7\\ $\pm$0.52\end{tabular}}           & {\begin{tabular}[c]{@{}l@{}}26.00\\ $\pm$0.50\end{tabular}}          & {\begin{tabular}[c]{@{}l@{}}22.43\\ $\pm$0.32\end{tabular}}          & {\begin{tabular}[c]{@{}l@{}}20.26\\ $\pm$0.42\end{tabular}}          & {\begin{tabular}[c]{@{}l@{}}18.22\\ $\pm$0.45\end{tabular}}          & {\begin{tabular}[c]{@{}l@{}}17.11\\ $\pm$0.44\end{tabular}}          & {\begin{tabular}[c]{@{}l@{}}31.95\\ $\pm$0.39\end{tabular}}          \\ \hline
{ICARL\cite{Rebuffi2017iCaRLIC}}                             & {\begin{tabular}[c]{@{}l@{}}60.70\\ $\pm$0.00\end{tabular}}          & {\begin{tabular}[c]{@{}l@{}}38.91\\ $\pm$0.56\end{tabular}}          & {\begin{tabular}[c]{@{}l@{}}30.65\\ $\pm$0.68\end{tabular}}          & {\begin{tabular}[c]{@{}l@{}}25.3\\ $\pm$0.59\end{tabular}}           & {\begin{tabular}[c]{@{}l@{}}21.46\\ $\pm$0.49\end{tabular}}          & {\begin{tabular}[c]{@{}l@{}}17.97\\ $\pm$0.39\end{tabular}}          & {\begin{tabular}[c]{@{}l@{}}16.38\\ $\pm$0.27\end{tabular}}          & {\begin{tabular}[c]{@{}l@{}}14.58\\ $\pm$0.12\end{tabular}}          & {\begin{tabular}[c]{@{}l@{}}13.77\\ $\pm$0.17\end{tabular}}          & {\begin{tabular}[c]{@{}l@{}}26.64\\ $\pm$0.36\end{tabular}}          \\ \hline
{Rebalance\cite{Hou2019LearningAU}}                         & {\begin{tabular}[c]{@{}l@{}}67.55\\ $\pm$0.00\end{tabular}}          & {\begin{tabular}[c]{@{}l@{}}44.89\\ $\pm$0.25\end{tabular}}          & {\begin{tabular}[c]{@{}l@{}}33.67\\ $\pm$0.18\end{tabular}}          & {\begin{tabular}[c]{@{}l@{}}29.04\\ $\pm$0.32\end{tabular}}          & {\begin{tabular}[c]{@{}l@{}}25.32\\ $\pm$0.38\end{tabular}}          & {\begin{tabular}[c]{@{}l@{}}22.19\\ $\pm$0.35\end{tabular}}          & {\begin{tabular}[c]{@{}l@{}}20.73\\ $\pm$0.69\end{tabular}}          & {\begin{tabular}[c]{@{}l@{}}18.88\\ $\pm$0.60\end{tabular}}          & {\begin{tabular}[c]{@{}l@{}}17.70\\ $\pm$0.61\end{tabular}}          & {\begin{tabular}[c]{@{}l@{}}31.11\\ $\pm$0.38\end{tabular}}          \\ \hline
{\textbf{FLOWER}}                   & {\textbf{\begin{tabular}[c]{@{}l@{}}75.70\\ $\pm$0.00\end{tabular}}} & {\textbf{\begin{tabular}[c]{@{}l@{}}52.66\\ $\pm$0.28\end{tabular}}} & {\textbf{\begin{tabular}[c]{@{}l@{}}41.67\\ $\pm$0.34\end{tabular}}} & {\textbf{\begin{tabular}[c]{@{}l@{}}33.88\\ $\pm$0.47\end{tabular}}} & {\textbf{\begin{tabular}[c]{@{}l@{}}28.64\\ $\pm$0.44\end{tabular}}} & {\textbf{\begin{tabular}[c]{@{}l@{}}24.63\\ $\pm$0.36\end{tabular}}} & {\textbf{\begin{tabular}[c]{@{}l@{}}22.00\\ $\pm$0.18\end{tabular}}} & {\textbf{\begin{tabular}[c]{@{}l@{}}19.67\\ $\pm$0.21\end{tabular}}} & {\textbf{\begin{tabular}[c]{@{}l@{}}18.21\\ $\pm$0.11\end{tabular}}} & {\textbf{\begin{tabular}[c]{@{}l@{}}35.23\\ $\pm$0.27\end{tabular}}} \\ \hline
\end{tabular}
% \end{tabular}
\caption{Complete numerical result on split MiniImagenet dataset with 60 and 20 base classes averaged across 5 times run, + indicates the results copied from TOPIC.}
\label{tab:full_miniimagenet}
\end{table*}

\begin{table*}
% \footnotesize
\small
\centering
% \begin{tabularx}{1.0\textwidth}{lXXXXXXXXX\fontsize{3}{5}r}
% \begin{tabularx}{1.0\textwidth}{lXXXXXXXXXr}
\begin{tabular}{lccccccccccccc}
\hline
\cline{1-11}
{}                                                           & \multicolumn{9}{c}{{\textbf{Session}}}         & {}                                            \\ \cline{2-10}
\multirow{-2}{*}{{\textbf{Method}}} & \centering{1}              & \centering{2}              & \centering{3}              & \centering{4}              & \centering{5}              & \centering{6}              & \centering{7}              & \centering{8}              & \centering{9}              & \multirow{-2}{*}{{\textbf{Avg}}} \\ \cline{1-11} \hline 
\multicolumn{11}{c}{{\textbf{Base classes = 60}}} \\ \hline
{Baseline\cite{Shi2021OvercomingCF}}                          & {\begin{tabular}[c]{@{}l@{}}72.20\\ $\pm$0.00\end{tabular}}          & {\begin{tabular}[c]{@{}l@{}}67.88\\ $\pm$0.28\end{tabular}}          & {\begin{tabular}[c]{@{}l@{}}64.06\\ $\pm$0.25\end{tabular}}          & {\begin{tabular}[c]{@{}l@{}}60.43\\ $\pm$0.37\end{tabular}}          & {\begin{tabular}[c]{@{}l@{}}57.28\\ $\pm$0.38\end{tabular}}          & {\begin{tabular}[c]{@{}l@{}}54.54\\ $\pm$0.36\end{tabular}}          & {\begin{tabular}[c]{@{}l@{}}52.83\\ $\pm$0.36\end{tabular}}          & {\begin{tabular}[c]{@{}l@{}}50.93\\ $\pm$0.23\end{tabular}}          & {\begin{tabular}[c]{@{}l@{}}48.80\\ $\pm$0.34\end{tabular}}          & {\begin{tabular}[c]{@{}l@{}}58.77\\ $\pm$0.29\end{tabular}}          \\ \hline
{F2M\cite{Shi2021OvercomingCF}}                               & {\begin{tabular}[c]{@{}l@{}}71.40\\ $\pm$0.00\end{tabular}}          & {\begin{tabular}[c]{@{}l@{}}66.65\\ $\pm$1.16\end{tabular}}          & {\begin{tabular}[c]{@{}l@{}}63.20\\ $\pm$1.04\end{tabular}}          & {\begin{tabular}[c]{@{}l@{}}59.54\\ $\pm$0.80\end{tabular}}          & {\begin{tabular}[c]{@{}l@{}}56.61\\ $\pm$0.74\end{tabular}}          & {\begin{tabular}[c]{@{}l@{}}54.08\\ $\pm$0.76\end{tabular}}          & {\begin{tabular}[c]{@{}l@{}}52.2\\ $\pm$0.66\end{tabular}}           & {\begin{tabular}[c]{@{}l@{}}50.49\\ $\pm$0.75\end{tabular}}          & {\begin{tabular}[c]{@{}l@{}}48.40\\ $\pm$0.65\end{tabular}}          & {\begin{tabular}[c]{@{}l@{}}58.06\\ $\pm$0.73\end{tabular}}          \\ \hline
{FSLL\cite{Mazumder2021FewShotLL}}                              & {\begin{tabular}[c]{@{}l@{}}72.52\\ $\pm$0.00\end{tabular}}          & {\begin{tabular}[c]{@{}l@{}}64.20\\ $\pm$0.67\end{tabular}}          & {\begin{tabular}[c]{@{}l@{}}59.60\\ $\pm$0.72\end{tabular}}          & {\begin{tabular}[c]{@{}l@{}}55.09\\ $\pm$0.53\end{tabular}}          & {\begin{tabular}[c]{@{}l@{}}52.85\\ $\pm$0.30\end{tabular}}          & {\begin{tabular}[c]{@{}l@{}}51.57\\ $\pm$0.10\end{tabular}}          & {\begin{tabular}[c]{@{}l@{}}51.21\\ $\pm$0.28\end{tabular}}          & {\begin{tabular}[c]{@{}l@{}}49.66\\ $\pm$0.29\end{tabular}}          & {\begin{tabular}[c]{@{}l@{}}47.86\\ $\pm$0.22\end{tabular}}          & {\begin{tabular}[c]{@{}l@{}}56.06\\ $\pm$0.35\end{tabular}}          \\ \hline
{ICARL\cite{Rebuffi2017iCaRLIC}}                             & {\begin{tabular}[c]{@{}l@{}}71.72\\ $\pm$0.00\end{tabular}}          & {\begin{tabular}[c]{@{}l@{}}64.86\\ $\pm$0.33\end{tabular}}          & {\begin{tabular}[c]{@{}l@{}}60.46\\ $\pm$0.23\end{tabular}}          & {\begin{tabular}[c]{@{}l@{}}56.61\\ $\pm$0.11\end{tabular}}          & {\begin{tabular}[c]{@{}l@{}}53.76\\ $\pm$0.15\end{tabular}}          & {\begin{tabular}[c]{@{}l@{}}51.10\\ $\pm$0.36\end{tabular}}          & {\begin{tabular}[c]{@{}l@{}}49.10\\ $\pm$0.53\end{tabular}}          & {\begin{tabular}[c]{@{}l@{}}46.95\\ $\pm$0.48\end{tabular}}          & {\begin{tabular}[c]{@{}l@{}}44.64\\ $\pm$0.56\end{tabular}}          & {\begin{tabular}[c]{@{}l@{}}55.47\\ $\pm$0.31\end{tabular}}          \\ \hline
{Rebalance\cite{Hou2019LearningAU}}                         & {\begin{tabular}[c]{@{}l@{}}74.57\\ $\pm$0.00\end{tabular}}          & {\begin{tabular}[c]{@{}l@{}}66.65\\ $\pm$0.35\end{tabular}}          & {\begin{tabular}[c]{@{}l@{}}60.96\\ $\pm$0.34\end{tabular}}          & {\begin{tabular}[c]{@{}l@{}}55.59\\ $\pm$0.28\end{tabular}}          & {\begin{tabular}[c]{@{}l@{}}50.87\\ $\pm$0.36\end{tabular}}          & {\begin{tabular}[c]{@{}l@{}}46.55\\ $\pm$0.64\end{tabular}}          & {\begin{tabular}[c]{@{}l@{}}43.82\\ $\pm$0.5\end{tabular}}           & {\begin{tabular}[c]{@{}l@{}}40.29\\ $\pm$0.60\end{tabular}}          & {\begin{tabular}[c]{@{}l@{}}37.23\\ $\pm$0.50\end{tabular}}          & {\begin{tabular}[c]{@{}l@{}}52.95\\ $\pm$0.40\end{tabular}}          \\ \hline
{ICARL+\cite{Rebuffi2017iCaRLIC}}                            & {\begin{tabular}[c]{@{}l@{}}64.10\\ $\pm$0.40\end{tabular}}          & {\begin{tabular}[c]{@{}l@{}}53.28\\ $\pm$0.57\end{tabular}}          & {\begin{tabular}[c]{@{}l@{}}41.69\\ $\pm$1.38\end{tabular}}          & {\begin{tabular}[c]{@{}l@{}}34.13\\ $\pm$0.91\end{tabular}}          & {\begin{tabular}[c]{@{}l@{}}27.93\\ $\pm$0.79\end{tabular}}          & {\begin{tabular}[c]{@{}l@{}}26.06\\ $\pm$0.50\end{tabular}}          & {\begin{tabular}[c]{@{}l@{}}20.41\\ $\pm$0.85\end{tabular}}          & {\begin{tabular}[c]{@{}l@{}}15.48\\ $\pm$0.95\end{tabular}}          & {\begin{tabular}[c]{@{}l@{}}13.73\\ $\pm$0.85\end{tabular}}          & {\begin{tabular}[c]{@{}l@{}}32.98\\ $\pm$0.80\end{tabular}}          \\ \hline
{EEIL+\cite{Castro2018EndtoEndIL}}                             & {\begin{tabular}[c]{@{}l@{}}64.10\\ $\pm$0.40\end{tabular}}          & {\begin{tabular}[c]{@{}l@{}}53.11\\ $\pm$0.51\end{tabular}}          & {\begin{tabular}[c]{@{}l@{}}42.71\\ $\pm$1.20\end{tabular}}          & {\begin{tabular}[c]{@{}l@{}}35.15\\ $\pm$0.81\end{tabular}}          & {\begin{tabular}[c]{@{}l@{}}28.96\\ $\pm$0.83\end{tabular}}          & {\begin{tabular}[c]{@{}l@{}}24.98\\ $\pm$0.59\end{tabular}}          & {\begin{tabular}[c]{@{}l@{}}21.01\\ $\pm$0.59\end{tabular}}          & {\begin{tabular}[c]{@{}l@{}}17.26\\ $\pm$0.80\end{tabular}}          & {\begin{tabular}[c]{@{}l@{}}15.85\\ $\pm$0.64\end{tabular}}          & {\begin{tabular}[c]{@{}l@{}}33.68\\ $\pm$0.71\end{tabular}}          \\ \hline
{Rebalance+\cite{Hou2019LearningAU}}                        & {\begin{tabular}[c]{@{}l@{}}64.10\\ $\pm$0.40\end{tabular}}          & {\begin{tabular}[c]{@{}l@{}}53.05\\ $\pm$0.55\end{tabular}}          & {\begin{tabular}[c]{@{}l@{}}43.96\\ $\pm$1.56\end{tabular}}          & {\begin{tabular}[c]{@{}l@{}}36.97\\ $\pm$0.83\end{tabular}}          & {\begin{tabular}[c]{@{}l@{}}31.61\\ $\pm$0.60\end{tabular}}          & {\begin{tabular}[c]{@{}l@{}}26.73\\ $\pm$0.65\end{tabular}}          & {\begin{tabular}[c]{@{}l@{}}21.23\\ $\pm$0.53\end{tabular}}          & {\begin{tabular}[c]{@{}l@{}}16.78\\ $\pm$1.00\end{tabular}}          & {\begin{tabular}[c]{@{}l@{}}13.54\\ $\pm$0.68\end{tabular}}          & {\begin{tabular}[c]{@{}l@{}}34.22\\ $\pm$0.76\end{tabular}}          \\ \hline
{TOPIC+\cite{Tao2020FewShotCL}}                            & {\begin{tabular}[c]{@{}l@{}}64.10\\ $\pm$0.40\end{tabular}}          & {\begin{tabular}[c]{@{}l@{}}55.88\\ $\pm$0.42\end{tabular}}          & {\begin{tabular}[c]{@{}l@{}}47.07\\ $\pm$1.18\end{tabular}}          & {\begin{tabular}[c]{@{}l@{}}45.16\\ $\pm$0.82\end{tabular}}          & {\begin{tabular}[c]{@{}l@{}}40.11\\ $\pm$0.79\end{tabular}}          & {\begin{tabular}[c]{@{}l@{}}36.38\\ $\pm$0.50\end{tabular}}          & {\begin{tabular}[c]{@{}l@{}}33.96\\ $\pm$0.69\end{tabular}}          & {\begin{tabular}[c]{@{}l@{}}31.55\\ $\pm$0.54\end{tabular}}          & {\begin{tabular}[c]{@{}l@{}}29.37\\ $\pm$0.80\end{tabular}}          & {\begin{tabular}[c]{@{}l@{}}42.62\\ $\pm$0.68\end{tabular}}          \\ \hline
{\textbf{FLOWER}}                   & {\textbf{\begin{tabular}[c]{@{}l@{}}73.40\\ $\pm$0.00\end{tabular}}} & {\textbf{\begin{tabular}[c]{@{}l@{}}68.98\\ $\pm$0.14\end{tabular}}} & {\textbf{\begin{tabular}[c]{@{}l@{}}64.98\\ $\pm$0.14\end{tabular}}} & {\textbf{\begin{tabular}[c]{@{}l@{}}61.20\\ $\pm$0.18\end{tabular}}} & {\textbf{\begin{tabular}[c]{@{}l@{}}57.88\\ $\pm$0.20\end{tabular}}} & {\textbf{\begin{tabular}[c]{@{}l@{}}55.14\\ $\pm$0.22\end{tabular}}} & {\textbf{\begin{tabular}[c]{@{}l@{}}53.28\\ $\pm$0.2\end{tabular}}}  & {\textbf{\begin{tabular}[c]{@{}l@{}}51.16\\ $\pm$0.29\end{tabular}}} & {\textbf{\begin{tabular}[c]{@{}l@{}}48.78\\ $\pm$0.24\end{tabular}}} & {\textbf{\begin{tabular}[c]{@{}l@{}}59.42\\ $\pm$0.18\end{tabular}}} \\ \hline
\multicolumn{11}{c}{{\textbf{Base classes = 20}}}         \\ \hline
{Baseline\cite{Shi2021OvercomingCF}}                          & {\begin{tabular}[c]{@{}l@{}}74.75\\ $\pm$0.00\end{tabular}}          & {\begin{tabular}[c]{@{}l@{}}54.39\\ $\pm$0.73\end{tabular}}          & {\begin{tabular}[c]{@{}l@{}}41.83\\ $\pm$0.49\end{tabular}}          & {\begin{tabular}[c]{@{}l@{}}35.24\\ $\pm$0.62\end{tabular}}          & {\begin{tabular}[c]{@{}l@{}}30.72\\ $\pm$0.59\end{tabular}}          & {\begin{tabular}[c]{@{}l@{}}27.67\\ $\pm$0.46\end{tabular}}          & {\begin{tabular}[c]{@{}l@{}}24.91\\ $\pm$0.45\end{tabular}}          & {\begin{tabular}[c]{@{}l@{}}22.82\\ $\pm$0.52\end{tabular}}          & {\begin{tabular}[c]{@{}l@{}}20.94\\ $\pm$0.39\end{tabular}}          & {\begin{tabular}[c]{@{}l@{}}37.03\\ $\pm$0.47\end{tabular}}          \\
{F2M\cite{Shi2021OvercomingCF}}                               & {\begin{tabular}[c]{@{}l@{}}73.40\\ $\pm$0.00\end{tabular}}          & {\begin{tabular}[c]{@{}l@{}}53.25\\ $\pm$0.57\end{tabular}}          & {\begin{tabular}[c]{@{}l@{}}42.10\\ $\pm$0.58\end{tabular}}          & {\begin{tabular}[c]{@{}l@{}}35.42\\ $\pm$0.58\end{tabular}}          & {\begin{tabular}[c]{@{}l@{}}31.03\\ $\pm$0.56\end{tabular}}          & {\begin{tabular}[c]{@{}l@{}}28.12\\ $\pm$0.45\end{tabular}}          & {\begin{tabular}[c]{@{}l@{}}24.95\\ $\pm$0.41\end{tabular}}          & {\begin{tabular}[c]{@{}l@{}}23.04\\ $\pm$0.48\end{tabular}}          & {\begin{tabular}[c]{@{}l@{}}21.38\\ $\pm$0.43\end{tabular}}          & {\begin{tabular}[c]{@{}l@{}}36.97\\ $\pm$0.45\end{tabular}}          \\ \hline
{FSLL\cite{Mazumder2021FewShotLL}}                              & {\begin{tabular}[c]{@{}l@{}}75.00\\ $\pm$0.00\end{tabular}}          & {\begin{tabular}[c]{@{}l@{}}52.76\\ $\pm$0.34\end{tabular}}          & {\begin{tabular}[c]{@{}l@{}}39.87\\ $\pm$0.62\end{tabular}}          & {\begin{tabular}[c]{@{}l@{}}33.29\\ $\pm$0.86\end{tabular}}          & {\begin{tabular}[c]{@{}l@{}}29.74\\ $\pm$0.62\end{tabular}}          & {\begin{tabular}[c]{@{}l@{}}26.73\\ $\pm$0.55\end{tabular}}          & {\begin{tabular}[c]{@{}l@{}}24.12\\ $\pm$0.5\end{tabular}}           & {\begin{tabular}[c]{@{}l@{}}22.22\\ $\pm$0.45\end{tabular}}          & {\begin{tabular}[c]{@{}l@{}}20.28\\ $\pm$0.35\end{tabular}}          & {\begin{tabular}[c]{@{}l@{}}36.00\\ $\pm$0.48\end{tabular}}          \\ \hline
{ICARL\cite{Rebuffi2017iCaRLIC}}                             & {\begin{tabular}[c]{@{}l@{}}76.85\\ $\pm$0.00\end{tabular}}          & {\begin{tabular}[c]{@{}l@{}}53.58\\ $\pm$0.68\end{tabular}}          & {\begin{tabular}[c]{@{}l@{}}41.51\\ $\pm$0.78\end{tabular}}          & {\begin{tabular}[c]{@{}l@{}}34.65\\ $\pm$0.73\end{tabular}}          & {\begin{tabular}[c]{@{}l@{}}30.22\\ $\pm$0.76\end{tabular}}          & {\begin{tabular}[c]{@{}l@{}}27.15\\ $\pm$0.51\end{tabular}}          & {\begin{tabular}[c]{@{}l@{}}23.73\\ $\pm$0.29\end{tabular}}          & {\begin{tabular}[c]{@{}l@{}}21.65\\ $\pm$0.30\end{tabular}}          & {\begin{tabular}[c]{@{}l@{}}19.62\\ $\pm$0.17\end{tabular}}          & {\begin{tabular}[c]{@{}l@{}}36.55\\ $\pm$0.47\end{tabular}}          \\ \hline
{Rebalance\cite{Hou2019LearningAU}}                         & {\begin{tabular}[c]{@{}l@{}}73.90\\ $\pm$0.00\end{tabular}}          & {\begin{tabular}[c]{@{}l@{}}49.27\\ $\pm$0.01\end{tabular}}          & {\begin{tabular}[c]{@{}l@{}}36.95\\ $\pm$0.00\end{tabular}}          & {\begin{tabular}[c]{@{}l@{}}31.73\\ $\pm$0.60\end{tabular}}          & {\begin{tabular}[c]{@{}l@{}}28.62\\ $\pm$0.58\end{tabular}}          & {\begin{tabular}[c]{@{}l@{}}26.68\\ $\pm$0.46\end{tabular}}          & {\begin{tabular}[c]{@{}l@{}}24.44\\ $\pm$0.31\end{tabular}}          & {\begin{tabular}[c]{@{}l@{}}22.62\\ $\pm$0.43\end{tabular}}          & {\begin{tabular}[c]{@{}l@{}}20.86\\ $\pm$0.32\end{tabular}}          & {\begin{tabular}[c]{@{}l@{}}35.01\\ $\pm$0.30\end{tabular}}          \\ \hline
{\textbf{FLOWER}}                   & {\textbf{\begin{tabular}[c]{@{}l@{}}83.20\\ $\pm$0.00\end{tabular}}} & {\textbf{\begin{tabular}[c]{@{}l@{}}58.93\\ $\pm$0.30\end{tabular}}} & {\textbf{\begin{tabular}[c]{@{}l@{}}46.01\\ $\pm$0.31\end{tabular}}} & {\textbf{\begin{tabular}[c]{@{}l@{}}38.56\\ $\pm$0.18\end{tabular}}} & {\textbf{\begin{tabular}[c]{@{}l@{}}33.48\\ $\pm$0.26\end{tabular}}} & {\textbf{\begin{tabular}[c]{@{}l@{}}29.54\\ $\pm$0.30\end{tabular}}} & {\textbf{\begin{tabular}[c]{@{}l@{}}26.49\\ $\pm$0.18\end{tabular}}} & {\textbf{\begin{tabular}[c]{@{}l@{}}24.40\\ $\pm$0.17\end{tabular}}} & {\textbf{\begin{tabular}[c]{@{}l@{}}22.27\\ $\pm$0.15\end{tabular}}} & {\textbf{\begin{tabular}[c]{@{}l@{}}40.32\\ $\pm$0.21\end{tabular}}}  \\ \hline
\end{tabular}
\caption{Complete numerical result on split CIFAR100 dataset with 60 and 20 base classes averaged across 5 times run, + indicates the results copied from TOPIC.}
\label{tab:full_cifar100}
\end{table*}


\begin{table*}[]
\footnotesize
% \scriptsize
\small
\centering
% \newcolumntype{A}{>{\left}p{0.145\textwidth}}
% \newcolumntype{S}{>{\fontsize{6}{6}}X}
% \newcolumntype{A}{>l{p{0.142\textwidth}}}
% \newcolumntype{B}{>{\hsize=.135\textwidth}X}
% % \begin{tabularx}{1.0\textwidth}{lXXXXXXXXXXX\fontsize{2}{2}r}
% \begin{tabularx}{1.0\textwidth}{BXXXXXXXXXXXr}
% \begin{tabularx}{1.0\textwidth}{ASSSSSSSSSSSr}
\begin{tabular}{lccccccccccccccc}
\hline
\cline{1-13}
{}                                  & \multicolumn{11}{c}{{\textbf{Session}}}       & {}                                                                \\
\multirow{-2}{*}{{\textbf{Method}}} & {1}                                                               & {2}                                                               & {3}                                                               & {4}                                                               & {5}                                                               & {6}                                                               & {7}                                                               & {8}                                                               & {9}                                                               & {10}                                                              & {11}                                                              & \multirow{-2}{*}{{\textbf{Avg}}}                                  \\ \hline
\multicolumn{13}{c}{{\textbf{Base classes = 100}}}    \\ \hline
{Baseline\cite{Shi2021OvercomingCF}}                          & {\begin{tabular}[c]{@{}l@{}}76.92\\ $\pm$0.00\end{tabular}}          & {\begin{tabular}[c]{@{}l@{}}72.83\\ $\pm$0.21\end{tabular}}          & {\begin{tabular}[c]{@{}l@{}}68.96\\ $\pm$0.28\end{tabular}}          & {\begin{tabular}[c]{@{}l@{}}64.74\\ $\pm$0.22\end{tabular}}          & {\begin{tabular}[c]{@{}l@{}}62.38\\ $\pm$0.34\end{tabular}}          & {\begin{tabular}[c]{@{}l@{}}59.63\\ $\pm$0.43\end{tabular}}          & {\begin{tabular}[c]{@{}l@{}}58.44\\ $\pm$0.41\end{tabular}}          & {\begin{tabular}[c]{@{}l@{}}57.25\\ $\pm$0.52\end{tabular}}          & {\begin{tabular}[c]{@{}l@{}}54.97\\ $\pm$0.40\end{tabular}}          & {\begin{tabular}[c]{@{}l@{}}54.33\\ $\pm$0.33\end{tabular}}          & {\begin{tabular}[c]{@{}l@{}}53.49\\ $\pm$0.47\end{tabular}}          & {\begin{tabular}[c]{@{}l@{}}62.18\\ $\pm$0.33\end{tabular}}          \\ \hline
{F2M\cite{Shi2021OvercomingCF}}                               & {\begin{tabular}[c]{@{}l@{}}77.41\\ $\pm$0.00\end{tabular}}          & {\begin{tabular}[c]{@{}l@{}}73.50\\ $\pm$0.17\end{tabular}}          & {\begin{tabular}[c]{@{}l@{}}69.52\\ $\pm$0.19\end{tabular}}          & {\begin{tabular}[c]{@{}l@{}}65.27\\ $\pm$0.26\end{tabular}}          & {\begin{tabular}[c]{@{}l@{}}63.07\\ $\pm$0.32\end{tabular}}          & {\begin{tabular}[c]{@{}l@{}}60.41\\ $\pm$0.26\end{tabular}}          & {\begin{tabular}[c]{@{}l@{}}59.20\\ $\pm$0.17\end{tabular}}          & {\begin{tabular}[c]{@{}l@{}}58.02\\ $\pm$0.17\end{tabular}}          & {\begin{tabular}[c]{@{}l@{}}55.89\\ $\pm$0.15\end{tabular}}          & {\begin{tabular}[c]{@{}l@{}}55.49\\ $\pm$0.13\end{tabular}}          & {\begin{tabular}[c]{@{}l@{}}54.51\\ $\pm$0.26\end{tabular}}          & {\begin{tabular}[c]{@{}l@{}}62.94\\ $\pm$0.19\end{tabular}}          \\ \hline
{FSLL\cite{Mazumder2021FewShotLL}}                              & {\begin{tabular}[c]{@{}l@{}}76.92\\ $\pm$0.00\end{tabular}}          & {\begin{tabular}[c]{@{}l@{}}70.58\\ $\pm$0.52\end{tabular}}          & {\begin{tabular}[c]{@{}l@{}}64.73\\ $\pm$0.18\end{tabular}}          & {\begin{tabular}[c]{@{}l@{}}57.77\\ $\pm$0.95\end{tabular}}          & {\begin{tabular}[c]{@{}l@{}}55.96\\ $\pm$0.81\end{tabular}}          & {\begin{tabular}[c]{@{}l@{}}54.34\\ $\pm$0.29\end{tabular}}          & {\begin{tabular}[c]{@{}l@{}}53.62\\ $\pm$0.61\end{tabular}}          & {\begin{tabular}[c]{@{}l@{}}53.04\\ $\pm$0.66\end{tabular}}          & {\begin{tabular}[c]{@{}l@{}}50.45\\ $\pm$0.58\end{tabular}}          & {\begin{tabular}[c]{@{}l@{}}50.36\\ $\pm$0.74\end{tabular}}          & {\begin{tabular}[c]{@{}l@{}}49.48\\ $\pm$0.66\end{tabular}}          & {\begin{tabular}[c]{@{}l@{}}57.93\\ $\pm$0.55\end{tabular}}          \\ \hline
{ICARL$\circ$\cite{Rebuffi2017iCaRLIC}}                             & {\begin{tabular}[c]{@{}l@{}}75.73\\ $\pm$0.00\end{tabular}}          & {\begin{tabular}[c]{@{}l@{}}69.97\\ $\pm$0.00\end{tabular}}          & {\begin{tabular}[c]{@{}l@{}}65.95\\ $\pm$0.00\end{tabular}}          & {\begin{tabular}[c]{@{}l@{}}61.27\\ $\pm$0.00\end{tabular}}          & {\begin{tabular}[c]{@{}l@{}}57.62\\ $\pm$0.00\end{tabular}}          & {\begin{tabular}[c]{@{}l@{}}55.50\\ $\pm$0.00\end{tabular}}          & {\begin{tabular}[c]{@{}l@{}}54.16\\ $\pm$0.00\end{tabular}}          & {\begin{tabular}[c]{@{}l@{}}53.37\\ $\pm$0.00\end{tabular}}          & {\begin{tabular}[c]{@{}l@{}}50.75\\ $\pm$0.00\end{tabular}}          & {\begin{tabular}[c]{@{}l@{}}50.35\\ $\pm$0.00\end{tabular}}          & {\begin{tabular}[c]{@{}l@{}}48.77\\ $\pm$0.00\end{tabular}}          & {\begin{tabular}[c]{@{}l@{}}58.49\\ $\pm$0.00\end{tabular}}          \\
{Rebalance\cite{Hou2019LearningAU}}                         & {\begin{tabular}[c]{@{}l@{}}74.83\\ $\pm$0.00\end{tabular}}          & {\begin{tabular}[c]{@{}l@{}}55.51\\ $\pm$0.58\end{tabular}}          & {\begin{tabular}[c]{@{}l@{}}48.36\\ $\pm$0.65\end{tabular}}          & {\begin{tabular}[c]{@{}l@{}}42.38\\ $\pm$0.89\end{tabular}}          & {\begin{tabular}[c]{@{}l@{}}36.98\\ $\pm$0.99\end{tabular}}          & {\begin{tabular}[c]{@{}l@{}}32.82\\ $\pm$0.91\end{tabular}}          & {\begin{tabular}[c]{@{}l@{}}30.15\\ $\pm$0.73\end{tabular}}          & {\begin{tabular}[c]{@{}l@{}}27.82\\ $\pm$0.48\end{tabular}}          & {\begin{tabular}[c]{@{}l@{}}25.96\\ $\pm$0.47\end{tabular}}          & {\begin{tabular}[c]{@{}l@{}}24.44\\ $\pm$0.59\end{tabular}}          & {\begin{tabular}[c]{@{}l@{}}22.83\\ $\pm$0.3\end{tabular}}           & {\begin{tabular}[c]{@{}l@{}}38.37\\ $\pm$0.60\end{tabular}}          \\ \hline
{ICARL+\cite{Rebuffi2017iCaRLIC}}                            & {\begin{tabular}[c]{@{}l@{}}68.68\\ $\pm$0.90\end{tabular}}          & {\begin{tabular}[c]{@{}l@{}}52.65\\ $\pm$0.93\end{tabular}}          & {\begin{tabular}[c]{@{}l@{}}48.61\\ $\pm$0.91\end{tabular}}          & {\begin{tabular}[c]{@{}l@{}}44.16\\ $\pm$0.89\end{tabular}}          & {\begin{tabular}[c]{@{}l@{}}36.62\\ $\pm$0.93\end{tabular}}          & {\begin{tabular}[c]{@{}l@{}}29.52\\ $\pm$0.97\end{tabular}}          & {\begin{tabular}[c]{@{}l@{}}27.83\\ $\pm$0.86\end{tabular}}          & {\begin{tabular}[c]{@{}l@{}}26.26\\ $\pm$0.88\end{tabular}}          & {\begin{tabular}[c]{@{}l@{}}24.01\\ $\pm$0.85\end{tabular}}          & {\begin{tabular}[c]{@{}l@{}}23.89\\ $\pm$0.92\end{tabular}}          & {\begin{tabular}[c]{@{}l@{}}21.16\\ $\pm$1.00\end{tabular}}          & {\begin{tabular}[c]{@{}l@{}}36.67\\ $\pm$0.91\end{tabular}}          \\ \hline
{EEIL+\cite{Castro2018EndtoEndIL}}                             & {\begin{tabular}[c]{@{}l@{}}68.68\\ $\pm$0.90\end{tabular}}          & {\begin{tabular}[c]{@{}l@{}}53.63\\ $\pm$1.09\end{tabular}}          & {\begin{tabular}[c]{@{}l@{}}47.91\\ $\pm$0.96\end{tabular}}          & {\begin{tabular}[c]{@{}l@{}}44.20\\ $\pm$0.98\end{tabular}}          & {\begin{tabular}[c]{@{}l@{}}36.30\\ $\pm$0.89\end{tabular}}          & {\begin{tabular}[c]{@{}l@{}}27.46\\ $\pm$0.97\end{tabular}}          & {\begin{tabular}[c]{@{}l@{}}25.93\\ $\pm$0.94\end{tabular}}          & {\begin{tabular}[c]{@{}l@{}}24.7\\ $\pm$1.04\end{tabular}}           & {\begin{tabular}[c]{@{}l@{}}23.95\\ $\pm$1.03\end{tabular}}          & {\begin{tabular}[c]{@{}l@{}}24.13\\ $\pm$0.89\end{tabular}}          & {\begin{tabular}[c]{@{}l@{}}22.11\\ $\pm$0.91\end{tabular}}          & {\begin{tabular}[c]{@{}l@{}}36.27\\ $\pm$0.96\end{tabular}}          \\ \hline
{Rebalance+\cite{Hou2019LearningAU}}                        & {\begin{tabular}[c]{@{}l@{}}68.68\\ $\pm$0.90\end{tabular}}          & {\begin{tabular}[c]{@{}l@{}}62.55\\ $\pm$0.93\end{tabular}}          & {\begin{tabular}[c]{@{}l@{}}50.33\\ $\pm$0.91\end{tabular}}          & {\begin{tabular}[c]{@{}l@{}}45.07\\ $\pm$0.94\end{tabular}}          & {\begin{tabular}[c]{@{}l@{}}38.25\\ $\pm$0.95\end{tabular}}          & {\begin{tabular}[c]{@{}l@{}}32.58\\ $\pm$0.98\end{tabular}}          & {\begin{tabular}[c]{@{}l@{}}28.71\\ $\pm$0.89\end{tabular}}          & {\begin{tabular}[c]{@{}l@{}}26.28\\ $\pm$0.88\end{tabular}}          & {\begin{tabular}[c]{@{}l@{}}23.80\\ $\pm$0.94\end{tabular}}          & {\begin{tabular}[c]{@{}l@{}}19.91\\ $\pm$0.96\end{tabular}}          & {\begin{tabular}[c]{@{}l@{}}17.82\\ $\pm$1.05\end{tabular}}          & {\begin{tabular}[c]{@{}l@{}}37.63\\ $\pm$0.94\end{tabular}}          \\ \hline
{TOPIC+\cite{Tao2020FewShotCL}}                            & {\begin{tabular}[c]{@{}l@{}}68.68\\ $\pm$0.90\end{tabular}}          & {\begin{tabular}[c]{@{}l@{}}62.49\\ $\pm$0.91\end{tabular}}          & {\begin{tabular}[c]{@{}l@{}}54.81\\ $\pm$0.92\end{tabular}}          & {\begin{tabular}[c]{@{}l@{}}49.99\\ $\pm$0.87\end{tabular}}          & {\begin{tabular}[c]{@{}l@{}}42.25\\ $\pm$0.85\end{tabular}}          & {\begin{tabular}[c]{@{}l@{}}41.40\\ $\pm$0.88\end{tabular}}          & {\begin{tabular}[c]{@{}l@{}}38.35\\ $\pm$0.96\end{tabular}}          & {\begin{tabular}[c]{@{}l@{}}35.36\\ $\pm$0.87\end{tabular}}          & {\begin{tabular}[c]{@{}l@{}}32.22\\ $\pm$0.90\end{tabular}}          & {\begin{tabular}[c]{@{}l@{}}28.31\\ $\pm$0.92\end{tabular}}          & {\begin{tabular}[c]{@{}l@{}}26.28\\ $\pm$0.91\end{tabular}}          & {\begin{tabular}[c]{@{}l@{}}43.65\\ $\pm$0.90\end{tabular}}          \\ \hline
{\textbf{FLOWER}}                   & {\textbf{\begin{tabular}[c]{@{}l@{}}79.02\\ $\pm$0.00\end{tabular}}} & {\textbf{\begin{tabular}[c]{@{}l@{}}75.77\\ $\pm$0.16\end{tabular}}} & {\textbf{\begin{tabular}[c]{@{}l@{}}72.01\\ $\pm$0.27\end{tabular}}} & {\textbf{\begin{tabular}[c]{@{}l@{}}67.96\\ $\pm$0.20\end{tabular}}} & {\textbf{\begin{tabular}[c]{@{}l@{}}65.99\\ $\pm$0.23\end{tabular}}} & {\textbf{\begin{tabular}[c]{@{}l@{}}63.38\\ $\pm$0.19\end{tabular}}} & {\textbf{\begin{tabular}[c]{@{}l@{}}62.14\\ $\pm$0.25\end{tabular}}} & {\textbf{\begin{tabular}[c]{@{}l@{}}61.12\\ $\pm$0.39\end{tabular}}} & {\textbf{\begin{tabular}[c]{@{}l@{}}58.96\\ $\pm$0.23\end{tabular}}} & {\textbf{\begin{tabular}[c]{@{}l@{}}58.52\\ $\pm$0.26\end{tabular}}} & {\textbf{\begin{tabular}[c]{@{}l@{}}57.49\\ $\pm$0.29\end{tabular}}} & {\textbf{\begin{tabular}[c]{@{}l@{}}65.67\\ $\pm$0.22\end{tabular}}} \\ \hline
\multicolumn{13}{c}{{\textbf{Base classes = 50}}}     \\ \hline
{Baseline\cite{Shi2021OvercomingCF}}                          & {\begin{tabular}[c]{@{}l@{}}77.83\\ $\pm$0.00\end{tabular}}          & {\begin{tabular}[c]{@{}l@{}}66.94\\ $\pm$0.40\end{tabular}}          & {\begin{tabular}[c]{@{}l@{}}61.18\\ $\pm$0.55\end{tabular}}          & {\begin{tabular}[c]{@{}l@{}}59.13\\ $\pm$0.81\end{tabular}}          & {\begin{tabular}[c]{@{}l@{}}54.85\\ $\pm$0.62\end{tabular}}          & {\begin{tabular}[c]{@{}l@{}}49.96\\ $\pm$0.59\end{tabular}}          & {\begin{tabular}[c]{@{}l@{}}46.73\\ $\pm$0.38\end{tabular}}          & {\begin{tabular}[c]{@{}l@{}}43.93\\ $\pm$0.33\end{tabular}}          & {\begin{tabular}[c]{@{}l@{}}42.30\\ $\pm$0.33\end{tabular}}          & {\begin{tabular}[c]{@{}l@{}}39.98\\ $\pm$0.37\end{tabular}}          & {\begin{tabular}[c]{@{}l@{}}39.74\\ $\pm$0.50\end{tabular}}          & {\begin{tabular}[c]{@{}l@{}}52.96\\ $\pm$0.44\end{tabular}}          \\ \hline
{F2M\cite{Shi2021OvercomingCF}}                               & {\begin{tabular}[c]{@{}l@{}}78.11\\ $\pm$0.00\end{tabular}}          & {\begin{tabular}[c]{@{}l@{}}68.52\\ $\pm$0.27\end{tabular}}          & {\begin{tabular}[c]{@{}l@{}}63.50\\ $\pm$0.23\end{tabular}}          & {\begin{tabular}[c]{@{}l@{}}61.61\\ $\pm$0.46\end{tabular}}          & {\begin{tabular}[c]{@{}l@{}}57.58\\ $\pm$0.37\end{tabular}}          & {\begin{tabular}[c]{@{}l@{}}52.64\\ $\pm$0.33\end{tabular}}          & {\begin{tabular}[c]{@{}l@{}}49.26\\ $\pm$0.48\end{tabular}}          & {\begin{tabular}[c]{@{}l@{}}46.43\\ $\pm$0.50\end{tabular}}          & {\begin{tabular}[c]{@{}l@{}}44.81\\ $\pm$0.43\end{tabular}}          & {\begin{tabular}[c]{@{}l@{}}42.71\\ $\pm$0.37\end{tabular}}          & {\begin{tabular}[c]{@{}l@{}}42.41\\ $\pm$0.53\end{tabular}}          & {\begin{tabular}[c]{@{}l@{}}55.23\\ $\pm$0.36\end{tabular}}          \\ \hline
{FSLL\cite{Mazumder2021FewShotLL}}                              & {\begin{tabular}[c]{@{}l@{}}77.61\\ $\pm$0.00\end{tabular}}          & {\begin{tabular}[c]{@{}l@{}}65.96\\ $\pm$0.64\end{tabular}}          & {\begin{tabular}[c]{@{}l@{}}60.37\\ $\pm$0.62\end{tabular}}          & {\begin{tabular}[c]{@{}l@{}}58.59\\ $\pm$0.92\end{tabular}}          & {\begin{tabular}[c]{@{}l@{}}55.96\\ $\pm$0.17\end{tabular}}          & {\begin{tabular}[c]{@{}l@{}}51.75\\ $\pm$0.28\end{tabular}}          & {\begin{tabular}[c]{@{}l@{}}48.35\\ $\pm$0.20\end{tabular}}          & {\begin{tabular}[c]{@{}l@{}}45.84\\ $\pm$0.56\end{tabular}}          & {\begin{tabular}[c]{@{}l@{}}44.92\\ $\pm$0.41\end{tabular}}          & {\begin{tabular}[c]{@{}l@{}}42.80\\ $\pm$0.50\end{tabular}}          & {\begin{tabular}[c]{@{}l@{}}42.62\\ $\pm$0.27\end{tabular}}          & {\begin{tabular}[c]{@{}l@{}}54.07\\ $\pm$0.42\end{tabular}}          \\ \hline
{ICARL$\circ$\cite{Rebuffi2017iCaRLIC}}                             & {\begin{tabular}[c]{@{}l@{}}75.88\\ $\pm$0.00\end{tabular}}          & {\begin{tabular}[c]{@{}l@{}}62.54\\ $\pm$0.00\end{tabular}}          & {\begin{tabular}[c]{@{}l@{}}57.70\\ $\pm$0.00\end{tabular}}          & {\begin{tabular}[c]{@{}l@{}}54.73\\ $\pm$0.00\end{tabular}}          & {\begin{tabular}[c]{@{}l@{}}49.16\\ $\pm$0.00\end{tabular}}          & {\begin{tabular}[c]{@{}l@{}}43.96\\ $\pm$0.00\end{tabular}}          & {\begin{tabular}[c]{@{}l@{}}40.84\\ $\pm$0.00\end{tabular}}          & {\begin{tabular}[c]{@{}l@{}}38.09\\ $\pm$0.00\end{tabular}}          & {\begin{tabular}[c]{@{}l@{}}36.63\\ $\pm$0.00\end{tabular}}          & {\begin{tabular}[c]{@{}l@{}}34.38\\ $\pm$0.00\end{tabular}}          & {\begin{tabular}[c]{@{}l@{}}34.79\\ $\pm$0.00\end{tabular}}          & {\begin{tabular}[c]{@{}l@{}}48.06\\ $\pm$0.00\end{tabular}}          \\ \hline
{Rebalance\cite{Hou2019LearningAU}}                         & {\begin{tabular}[c]{@{}l@{}}74.73\\ $\pm$0.00\end{tabular}}          & {\begin{tabular}[c]{@{}l@{}}60.91\\ $\pm$0.63\end{tabular}}          & {\begin{tabular}[c]{@{}l@{}}56.29\\ $\pm$0.39\end{tabular}}          & {\begin{tabular}[c]{@{}l@{}}53.93\\ $\pm$1.01\end{tabular}}          & {\begin{tabular}[c]{@{}l@{}}48.31\\ $\pm$0.35\end{tabular}}          & {\begin{tabular}[c]{@{}l@{}}42.49\\ $\pm$0.57\end{tabular}}          & {\begin{tabular}[c]{@{}l@{}}37.40\\ $\pm$0.81\end{tabular}}          & {\begin{tabular}[c]{@{}l@{}}33.42\\ $\pm$0.26\end{tabular}}          & {\begin{tabular}[c]{@{}l@{}}31.32\\ $\pm$0.47\end{tabular}}          & {\begin{tabular}[c]{@{}l@{}}29.29\\ $\pm$0.65\end{tabular}}          & {\begin{tabular}[c]{@{}l@{}}27.93\\ $\pm$0.40\end{tabular}}          & {\begin{tabular}[c]{@{}l@{}}45.09\\ $\pm$0.5\end{tabular}}           \\ \hline
{\textbf{FLOWER}}                   & {\textbf{\begin{tabular}[c]{@{}l@{}}79.63\\ $\pm$0.00\end{tabular}}} & {\textbf{\begin{tabular}[c]{@{}l@{}}71.14\\ $\pm$0.38\end{tabular}}} & {\textbf{\begin{tabular}[c]{@{}l@{}}66.18\\ $\pm$0.61\end{tabular}}} & {\textbf{\begin{tabular}[c]{@{}l@{}}64.22\\ $\pm$0.55\end{tabular}}} & {\textbf{\begin{tabular}[c]{@{}l@{}}60.03\\ $\pm$0.43\end{tabular}}} & {\textbf{\begin{tabular}[c]{@{}l@{}}55.17\\ $\pm$0.24\end{tabular}}} & {\textbf{\begin{tabular}[c]{@{}l@{}}51.74\\ $\pm$0.14\end{tabular}}} & {\textbf{\begin{tabular}[c]{@{}l@{}}49.13\\ $\pm$0.31\end{tabular}}} & {\textbf{\begin{tabular}[c]{@{}l@{}}47.79\\ $\pm$0.47\end{tabular}}} & {\textbf{\begin{tabular}[c]{@{}l@{}}45.68\\ $\pm$0.37\end{tabular}}} & {\textbf{\begin{tabular}[c]{@{}l@{}}45.29\\ $\pm$0.49\end{tabular}}} & {\textbf{\begin{tabular}[c]{@{}l@{}}57.82\\ $\pm$0.36\end{tabular}}} \\ \hline
\end{tabular} 
\caption{Complete numerical result on split CUB 2011 dataset with 100 and 50 base classes averaged across 5 times run, + indicates the results copied from TOPIC, $\circ$ indicates the method is run 1 time due to system crash.}
\label{tab:full_cub}
\end{table*}

%\begin{appendices}
\section{Complete Numerical Results of 1-Shot Experiments}   
\begin{table*}[]
\centering
% \footnotesize
\small
% \begin{tabularx}{1.0\textwidth}{lXXXXXXXXXXXX\fontsize{3}{5}r}
% \begin{tabularx}{1.0\textwidth}{lXXXXXXXXXXXXr}
\begin{tabular}{lccccccccccccc}
\hline
\multicolumn{1}{c}{{}}                                  & \multicolumn{9}{c}{{\textbf{Session}}}                                        & \multicolumn{1}{c}{{}}                                            \\
\multicolumn{1}{c}{\multirow{-2}{*}{{\textbf{Method}}}} & \multicolumn{1}{c}{{1}}                                           & \multicolumn{1}{c}{{2}}                                           & \multicolumn{1}{c}{{3}}                                           & \multicolumn{1}{c}{{4}}                                           & \multicolumn{1}{c}{{5}}                                           & \multicolumn{1}{c}{{6}}                                           & \multicolumn{1}{c}{{7}}                                           & \multicolumn{1}{c}{{8}}                                           & \multicolumn{1}{c}{{9}}                                           & \multicolumn{1}{c}{\multirow{-2}{*}{{\textbf{Avg}}}}              \\ \hline
% {Baseline}                 & {66.78}          & {61.65}          & {57.26}          & {53.50}          & {50.22}          & {47.30}          & {44.70}          & {42.42}          & {40.51}          & {51.59}                 \\
% {F2M}                      & {66.07}          & {60.92}          & {56.51}          & {52.78}          & {49.52}          & {46.61}          & {44.03}          & {41.81}          & {39.86}          & {50.90}                 \\
% {FSLL}                     & {66.98}          & {52.53}          & {48.75}          & {46.69}          & {44.54}          & {42.11}          & {40.43}          & {38.82}          & {37.58}          & {46.49}                 \\
% {ICARL}                    & {66.05}          & {1.54}           & {1.43}           & {1.33}           & {1.25}           & {1.18}           & {1.11}           & {1.05}           & {1.00}           & {8.44}                  \\
% {Rebalance}                & {66.45}          & {61.33}          & {56.95}          & {53.15}          & {49.83}          & {46.90}          & {44.29}          & {41.96}          & {39.86}          & {51.19}                 \\
% {FLOWER}                   & {\textbf{68.83}} & {\textbf{63.50}} & {\textbf{58.92}} & {\textbf{55.14}} & {\textbf{51.78}} & {\textbf{48.66}} & {\textbf{45.93}} & {\textbf{43.58}} & {\textbf{41.67}} & {\textbf{53.11}} \\ \hline
{Baseline\cite{Shi2021OvercomingCF}}                                              & {\begin{tabular}[c]{@{}l@{}}66.78\\ $\pm$0.00\end{tabular}}          & {\begin{tabular}[c]{@{}l@{}}61.65\\ $\pm$0.08\end{tabular}}          & {\begin{tabular}[c]{@{}l@{}}57.26\\ $\pm$0.08\end{tabular}}          & {\begin{tabular}[c]{@{}l@{}}53.50\\ $\pm$0.06\end{tabular}}           & {\begin{tabular}[c]{@{}l@{}}50.22\\ $\pm$0.07\end{tabular}}          & {\begin{tabular}[c]{@{}l@{}}47.30\\ $\pm$0.08\end{tabular}}          & {\begin{tabular}[c]{@{}l@{}}44.70\\ $\pm$0.08\end{tabular}}           & {\begin{tabular}[c]{@{}l@{}}42.42\\ $\pm$0.05\end{tabular}}          & {\begin{tabular}[c]{@{}l@{}}40.51\\ $\pm$0.15\end{tabular}}          & {\begin{tabular}[c]{@{}l@{}}51.59\\ $\pm$0.07\end{tabular}}          \\ \hline
{F2M\cite{Shi2021OvercomingCF}}                                                   & {\begin{tabular}[c]{@{}l@{}}66.07\\ $\pm$0.00\end{tabular}}          & {\begin{tabular}[c]{@{}l@{}}60.92\\ $\pm$0.05\end{tabular}}          & {\begin{tabular}[c]{@{}l@{}}56.51\\ $\pm$0.05\end{tabular}}          & {\begin{tabular}[c]{@{}l@{}}52.78\\ $\pm$0.07\end{tabular}}          & {\begin{tabular}[c]{@{}l@{}}49.52\\ $\pm$0.10\end{tabular}}          & {\begin{tabular}[c]{@{}l@{}}46.61\\ $\pm$0.09\end{tabular}}          & {\begin{tabular}[c]{@{}l@{}}44.03\\ $\pm$0.11\end{tabular}}          & {\begin{tabular}[c]{@{}l@{}}41.81\\ $\pm$0.08\end{tabular}}          & {\begin{tabular}[c]{@{}l@{}}39.86\\ $\pm$0.15\end{tabular}}          & {\begin{tabular}[c]{@{}l@{}}50.90\\ $\pm$0.08\end{tabular}}           \\ \hline
{FSLL\cite{Mazumder2021FewShotLL}}                                                  & {\begin{tabular}[c]{@{}l@{}}66.98\\ $\pm$0.00\end{tabular}}          & {\begin{tabular}[c]{@{}l@{}}52.53\\ $\pm$0.72\end{tabular}}          & {\begin{tabular}[c]{@{}l@{}}48.75\\ $\pm$1.07\end{tabular}}          & {\begin{tabular}[c]{@{}l@{}}46.69\\ $\pm$1.13\end{tabular}}          & {\begin{tabular}[c]{@{}l@{}}44.54\\ $\pm$0.89\end{tabular}}          & {\begin{tabular}[c]{@{}l@{}}42.11\\ $\pm$0.61\end{tabular}}          & {\begin{tabular}[c]{@{}l@{}}40.43\\ $\pm$0.58\end{tabular}}          & {\begin{tabular}[c]{@{}l@{}}38.82\\ $\pm$0.5\end{tabular}}           & {\begin{tabular}[c]{@{}l@{}}37.58\\ $\pm$0.41\end{tabular}}          & {\begin{tabular}[c]{@{}l@{}}46.49\\ $\pm$0.66\end{tabular}}          \\ \hline
{ICARL\cite{Rebuffi2017iCaRLIC}}                                                 & {\begin{tabular}[c]{@{}l@{}}66.05\\ $\pm$0.00\end{tabular}}          & {\begin{tabular}[c]{@{}l@{}}1.54\\ $\pm$0.00\end{tabular}}           & {\begin{tabular}[c]{@{}l@{}}1.43\\ $\pm$0.00\end{tabular}}           & {\begin{tabular}[c]{@{}l@{}}1.33\\ $\pm$0.00\end{tabular}}           & {\begin{tabular}[c]{@{}l@{}}1.25\\ $\pm$0,00\end{tabular}}           & {\begin{tabular}[c]{@{}l@{}}1.18\\ $\pm$0.00\end{tabular}}           & {\begin{tabular}[c]{@{}l@{}}1.11\\ $\pm$0.00\end{tabular}}           & {\begin{tabular}[c]{@{}l@{}}1.05\\ $\pm$0.00\end{tabular}}           & {\begin{tabular}[c]{@{}l@{}}1.00\\ $\pm$0.00\end{tabular}}           & {\begin{tabular}[c]{@{}l@{}}8.44\\ $\pm$0.00\end{tabular}}           \\ \hline
{Rebalance\cite{Hou2019LearningAU}}                                             & {\begin{tabular}[c]{@{}l@{}}66.45\\ $\pm$0.00\end{tabular}}          & {\begin{tabular}[c]{@{}l@{}}61.33\\ $\pm$0.02\end{tabular}}          & {\begin{tabular}[c]{@{}l@{}}56.95\\ $\pm$0.02\end{tabular}}          & {\begin{tabular}[c]{@{}l@{}}53.15\\ $\pm$0.01\end{tabular}}          & {\begin{tabular}[c]{@{}l@{}}49.83\\ $\pm$0.01\end{tabular}}          & {\begin{tabular}[c]{@{}l@{}}46.90\\ $\pm$0.01\end{tabular}}          & {\begin{tabular}[c]{@{}l@{}}44.29\\ $\pm$0.01\end{tabular}}          & {\begin{tabular}[c]{@{}l@{}}41.96\\ $\pm$0.01\end{tabular}}          & {\begin{tabular}[c]{@{}l@{}}39.86\\ $\pm$0.01\end{tabular}}          & {\begin{tabular}[c]{@{}l@{}}51.19\\ $\pm$0.01\end{tabular}}          \\ \hline
{\textbf{FLOWER}}                                       & {\textbf{\begin{tabular}[c]{@{}l@{}}68.83\\ $\pm$0.00\end{tabular}}} & {\textbf{\begin{tabular}[c]{@{}l@{}}63.50\\ $\pm$0.11\end{tabular}}}  & {\textbf{\begin{tabular}[c]{@{}l@{}}58.92\\ $\pm$0.15\end{tabular}}} & {\textbf{\begin{tabular}[c]{@{}l@{}}55.14\\ $\pm$0.16\end{tabular}}} & {\textbf{\begin{tabular}[c]{@{}l@{}}51.78\\ $\pm$0.17\end{tabular}}} & {\textbf{\begin{tabular}[c]{@{}l@{}}48.66\\ $\pm$0.14\end{tabular}}} & {\textbf{\begin{tabular}[c]{@{}l@{}}45.93\\ $\pm$0.16\end{tabular}}} & {\textbf{\begin{tabular}[c]{@{}l@{}}43.58\\ $\pm$0.18\end{tabular}}} & {\textbf{\begin{tabular}[c]{@{}l@{}}41.67\\ $\pm$0.27\end{tabular}}} & {\textbf{\begin{tabular}[c]{@{}l@{}}53.11\\ $\pm$0.15\end{tabular}}} \\ \hline
\end{tabular}
\caption{Classification accuracy with 1-shot setting on 60 base classes MiniImageNet  dataset. This table is the detailed version of table \ref{tab:1shot} in main paper for MiniImagenet dataset.}
\label{tab:1shot_miniimagenet}
\end{table*}

\begin{table*}[]
\centering
% \footnotesize
\small
% \begin{tabularx}{1.0\textwidth}{lXXXXXXXXXXXX\fontsize{3}{5}r}
% \begin{tabularx}{1.0\textwidth}{lXXXXXXXXXXXXr}
\begin{tabular}{lccccccccccccc}
\hline
\multicolumn{1}{c}{{}}                                  & \multicolumn{9}{c}{{\textbf{Session}}}                                        & \multicolumn{1}{c}{{}}                                            \\
\multicolumn{1}{c}{\multirow{-2}{*}{{\textbf{Method}}}} & \multicolumn{1}{c}{{1}}                                           & \multicolumn{1}{c}{{2}}                                           & \multicolumn{1}{c}{{3}}                                           & \multicolumn{1}{c}{{4}}                                           & \multicolumn{1}{c}{{5}}                                           & \multicolumn{1}{c}{{6}}                                           & \multicolumn{1}{c}{{7}}                                           & \multicolumn{1}{c}{{8}}                                           & \multicolumn{1}{c}{{9}}                                           & \multicolumn{1}{c}{\multirow{-2}{*}{{\textbf{Avg}}}}              \\ \hline
% {Baseline}                 & {72.20}          & {67.39}          & {62.95}          & {59.15}          & {55.73}          & {52.57}          & {50.01}          & {47.72}          & {45.36}          & {57.01}                 \\
% {F2M}                      & {71.40}          & {66.50}          & {62.02}          & {58.10}          & {54.70}          & {51.60}          & {48.94}          & {46.81}          & {44.57}          & {56.07}                 \\
% {FSLL}                     & {72.52}          & {59.22}          & {55.84}          & {52.55}          & {50.25}          & {48.78}          & {47.56}          & {45.65}          & {43.61}          & {52.89}                 \\
% {ICARL}                    & {71.72}          & {1.54}           & {1.43}           & {1.33}           & {1.25}           & {1.18}           & {1.11}           & {1.05}           & {1.00}           & {9.07}                  \\
% {Rebalance}                & {\textbf{74.57}} & {\textbf{68.83}} & {\textbf{63.91}} & {\textbf{59.65}} & {\textbf{55.92}} & {52.62}          & {49.70}          & {47.08}          & {44.72}          & {\textbf{57.44}}        \\
% {FLOWER}                   & {73.40}          & {68.47}          & {63.76}          & {59.59}          & {55.86}          & {\textbf{52.72}} & {\textbf{50.14}} & {\textbf{47.68}} & {\textbf{45.27}} & {\textbf{57.43}}  \\ \hline    
{Baseline\cite{Shi2021OvercomingCF}}                                              & {\begin{tabular}[c]{@{}l@{}}72.20\\ $\pm$0.00\end{tabular}}          & {\begin{tabular}[c]{@{}l@{}}67.39\\ $\pm$0.22\end{tabular}}          & {\begin{tabular}[c]{@{}l@{}}62.95\\ $\pm$0.26\end{tabular}}          & {\begin{tabular}[c]{@{}l@{}}59.15\\ $\pm$0.29\end{tabular}}          & {\begin{tabular}[c]{@{}l@{}}55.73\\ $\pm$0.25\end{tabular}}          & {\begin{tabular}[c]{@{}l@{}}52.57\\ $\pm$0.31\end{tabular}}          & {\begin{tabular}[c]{@{}l@{}}50.01\\ $\pm$0.27\end{tabular}}          & {\begin{tabular}[c]{@{}l@{}}47.72\\ $\pm$0.36\end{tabular}}          & {\begin{tabular}[c]{@{}l@{}}45.36\\ $\pm$0.40\end{tabular}}          & {\begin{tabular}[c]{@{}l@{}}57.01\\ $\pm$0.26\end{tabular}}          \\ \hline
{F2M\cite{Shi2021OvercomingCF}}                                                   & {\begin{tabular}[c]{@{}l@{}}71.40\\ $\pm$0.00\end{tabular}}          & {\begin{tabular}[c]{@{}l@{}}66.50\\ $\pm$0.16\end{tabular}}          & {\begin{tabular}[c]{@{}l@{}}62.02\\ $\pm$0.17\end{tabular}}          & {\begin{tabular}[c]{@{}l@{}}58.10\\ $\pm$0.17\end{tabular}}          & {\begin{tabular}[c]{@{}l@{}}54.70\\ $\pm$0.12\end{tabular}}          & {\begin{tabular}[c]{@{}l@{}}51.60\\ $\pm$0.15\end{tabular}}          & {\begin{tabular}[c]{@{}l@{}}48.94\\ $\pm$0.14\end{tabular}}          & {\begin{tabular}[c]{@{}l@{}}46.81\\ $\pm$0.29\end{tabular}}          & {\begin{tabular}[c]{@{}l@{}}44.57\\ $\pm$0.23\end{tabular}}          & {\begin{tabular}[c]{@{}l@{}}56.07\\ $\pm$0.16\end{tabular}}          \\ \hline
{FSLL\cite{Mazumder2021FewShotLL}}                                                  & {\begin{tabular}[c]{@{}l@{}}72.52\\ $\pm$0.00\end{tabular}}          & {\begin{tabular}[c]{@{}l@{}}59.22\\ $\pm$1.23\end{tabular}}          & {\begin{tabular}[c]{@{}l@{}}55.84\\ $\pm$0.86\end{tabular}}          & {\begin{tabular}[c]{@{}l@{}}52.55\\ $\pm$0.94\end{tabular}}          & {\begin{tabular}[c]{@{}l@{}}50.25\\ $\pm$0.91\end{tabular}}          & {\begin{tabular}[c]{@{}l@{}}48.78\\ $\pm$0.77\end{tabular}}          & {\begin{tabular}[c]{@{}l@{}}47.56\\ $\pm$0.74\end{tabular}}          & {\begin{tabular}[c]{@{}l@{}}45.65\\ $\pm$0.64\end{tabular}}          & {\begin{tabular}[c]{@{}l@{}}43.61\\ $\pm$0.49\end{tabular}}          & {\begin{tabular}[c]{@{}l@{}}52.89\\ $\pm$0.73\end{tabular}}          \\ \hline
{ICARL\cite{Rebuffi2017iCaRLIC}}                                                 & {\begin{tabular}[c]{@{}l@{}}71.72\\ $\pm$0.00\end{tabular}}          & {\begin{tabular}[c]{@{}l@{}}1.54\\ $\pm$0.00\end{tabular}}           & {\begin{tabular}[c]{@{}l@{}}1.43\\ $\pm$0.00\end{tabular}}           & {\begin{tabular}[c]{@{}l@{}}1.33\\ $\pm$0.00\end{tabular}}           & {\begin{tabular}[c]{@{}l@{}}1.25\\ $\pm$0.00\end{tabular}}           & {\begin{tabular}[c]{@{}l@{}}1.18\\ $\pm$0.00\end{tabular}}           & {\begin{tabular}[c]{@{}l@{}}1.11\\ $\pm$0.00\end{tabular}}           & {\begin{tabular}[c]{@{}l@{}}1.05\\ $\pm$0.00\end{tabular}}           & {\begin{tabular}[c]{@{}l@{}}1.00\\ $\pm$0.00\end{tabular}}           & {\begin{tabular}[c]{@{}l@{}}9.07\\ $\pm$0.00\end{tabular}}           \\ \hline
{Rebalance\cite{Hou2019LearningAU}}                                             & {\begin{tabular}[c]{@{}l@{}}74.57\\ $\pm$0.00\end{tabular}}          & {\begin{tabular}[c]{@{}l@{}}68.83\\ $\pm$0.01\end{tabular}}          & {\begin{tabular}[c]{@{}l@{}}63.91\\ $\pm$0.01\end{tabular}}          & {\begin{tabular}[c]{@{}l@{}}59.65\\ $\pm$0.01\end{tabular}}          & {\begin{tabular}[c]{@{}l@{}}55.92\\ $\pm$0.01\end{tabular}}          & {\begin{tabular}[c]{@{}l@{}}52.62\\ $\pm$0.01\end{tabular}}          & {\begin{tabular}[c]{@{}l@{}}49.7\\ $\pm$0.01\end{tabular}}           & {\begin{tabular}[c]{@{}l@{}}47.08\\ $\pm$0.00\end{tabular}}          & {\begin{tabular}[c]{@{}l@{}}44.72\\ $\pm$0.00\end{tabular}}          & {\textbf{\begin{tabular}[c]{@{}l@{}}57.44\\ $\pm$0.01\end{tabular}}} \\ \hline
{\textbf{FLOWER}}                                       & {\textbf{\begin{tabular}[c]{@{}l@{}}73.40\\ $\pm$0.00\end{tabular}}} & {\textbf{\begin{tabular}[c]{@{}l@{}}68.47\\ $\pm$0.16\end{tabular}}} & {\textbf{\begin{tabular}[c]{@{}l@{}}63.76\\ $\pm$0.23\end{tabular}}} & {\textbf{\begin{tabular}[c]{@{}l@{}}59.59\\ $\pm$0.27\end{tabular}}} & {\textbf{\begin{tabular}[c]{@{}l@{}}55.86\\ $\pm$0.29\end{tabular}}} & {\textbf{\begin{tabular}[c]{@{}l@{}}52.72\\ $\pm$0.27\end{tabular}}} & {\textbf{\begin{tabular}[c]{@{}l@{}}50.14\\ $\pm$0.24\end{tabular}}} & {\textbf{\begin{tabular}[c]{@{}l@{}}47.68\\ $\pm$0.29\end{tabular}}} & {\textbf{\begin{tabular}[c]{@{}l@{}}45.27\\ $\pm$0.26\end{tabular}}} & {\textbf{\begin{tabular}[c]{@{}l@{}}57.43\\ $\pm$0.22\end{tabular}}} \\ \hline
\end{tabular}
\caption{Classification accuracy with 1-shot setting on 60 base classes CIFAR-100 dataset. This table is detailed version of table \ref{tab:1shot} in main paper for CIFAR-100 dataset.}
\label{tab:1shot_cifar100}
\end{table*}

\begin{table*}[ht]
\centering
% \footnotesize
\small
% \begin{tabularx}{1.0\textwidth}{lXXXXXXXXXXXX\fontsize{3}{5}r}
% \newcolumntype{B}{>{\hsize=.13\textwidth}X}
% \begin{tabularx}{1.0\textwidth}{BXXXXXXXXXXXXr}
\begin{tabular}{lccccccccccccccc}
\hline
{}                         & \multicolumn{11}{c}{\textbf{Session}}                                       & {}                      \\ \cline{2-12} 
\multirow{-2}{*}{\textbf{Method}} & {1}              & {2}              & {3}              & {4}              & {5}              & {6}              & {7}              & {8}              & {9}              & {10}             & {11}             & \multirow{-2}{*}{\textbf{Avg}} \\ \hline
% {Baseline}                 & {76.92}          & {70.89}          & {65.79}          & {61.16}          & {57.29}          & {53.87}          & {51.16}          & {49.01}          & {46.71}          & {44.79}          & {43.13}          & {57.76}                 \\
% {F2M}                      & {77.41}          & {71.38}          & {65.87}          & {61.20}          & {57.23}          & {53.81}          & {51.01}          & {48.66}          & {46.35}          & {44.40}          & {42.55}          & {57.73}                 \\
% {FSLL}                     & {76.92}          & {66.97}          & {59.78}          & {52.62}          & {50.49}          & {48.54}          & {46.49}          & {44.35}          & {41.97}          & {40.46}          & {38.79}          & {52.86}                 \\
% {ICARL}                    & {75.73}          & {0.95}           & {0.87}           & {0.80}           & {0.74}           & {0.69}           & {0.65}           & {0.61}           & {0.58}           & {0.55}           & {0.52}           & {8.22}                  \\
% {Rebalance}                & {74.83}          & {68.18}          & {47.50}          & {41.87}          & {37.27}          & {33.49}          & {29.77}          & {26.78}          & {24.21}          & {22.28}          & {20.43}          & {40.62}                 \\
% {FLOWER}                   & {\textbf{79.02}} & {\textbf{72.73}} & {\textbf{67.29}} & {\textbf{62.74}} & {\textbf{58.82}} & {\textbf{55.43}} & {\textbf{52.63}} & {\textbf{50.18}} & {\textbf{47.77}} & {\textbf{46.05}} & {\textbf{44.26}} & {\textbf{59.27}} \\ \hline
{Baseline\cite{Shi2021OvercomingCF}}                                              & {\begin{tabular}[c]{@{}l@{}}76.92\\ $\pm$0.00\end{tabular}}          & {\begin{tabular}[c]{@{}l@{}}70.89\\ $\pm$0.15\end{tabular}}          & {\begin{tabular}[c]{@{}l@{}}65.79\\ $\pm$0.33\end{tabular}}          & {\begin{tabular}[c]{@{}l@{}}61.16\\ $\pm$0.2\end{tabular}}           & {\begin{tabular}[c]{@{}l@{}}57.29\\ $\pm$0.25\end{tabular}}          & {\begin{tabular}[c]{@{}l@{}}53.87\\ $\pm$0.05\end{tabular}}          & {\begin{tabular}[c]{@{}l@{}}51.16\\ $\pm$0.18\end{tabular}}          & {\begin{tabular}[c]{@{}l@{}}49.01\\ $\pm$0.16\end{tabular}}          & {\begin{tabular}[c]{@{}l@{}}46.71\\ $\pm$0.4\end{tabular}}           & {\begin{tabular}[c]{@{}l@{}}44.79\\ $\pm$0.32\end{tabular}}          & {\begin{tabular}[c]{@{}l@{}}43.13\\ $\pm$0.4\end{tabular}}           & {\begin{tabular}[c]{@{}l@{}}56.43\\ $\pm$0.22\end{tabular}}          \\ \hline
{F2M\cite{Shi2021OvercomingCF}}                                                   & {\begin{tabular}[c]{@{}l@{}}77.41\\ $\pm$0.00\end{tabular}}          & {\begin{tabular}[c]{@{}l@{}}71.38\\ $\pm$0.14\end{tabular}}          & {\begin{tabular}[c]{@{}l@{}}65.87\\ $\pm$0.28\end{tabular}}          & {\begin{tabular}[c]{@{}l@{}}61.2\\ $\pm$0.25\end{tabular}}           & {\begin{tabular}[c]{@{}l@{}}57.23\\ $\pm$0.18\end{tabular}}          & {\begin{tabular}[c]{@{}l@{}}53.81\\ $\pm$0.2\end{tabular}}           & {\begin{tabular}[c]{@{}l@{}}51.01\\ $\pm$0.19\end{tabular}}          & {\begin{tabular}[c]{@{}l@{}}48.66\\ $\pm$0.14\end{tabular}}          & {\begin{tabular}[c]{@{}l@{}}46.35\\ $\pm$0.15\end{tabular}}          & {\begin{tabular}[c]{@{}l@{}}44.4\\ $\pm$0.15\end{tabular}}           & {\begin{tabular}[c]{@{}l@{}}42.55\\ $\pm$0.23\end{tabular}}          & {\begin{tabular}[c]{@{}l@{}}56.35\\ $\pm$0.17\end{tabular}}          \\ \hline
{FSLL\cite{Mazumder2021FewShotLL}}                                                  & {\begin{tabular}[c]{@{}l@{}}76.92\\ $\pm$0.00\end{tabular}}          & {\begin{tabular}[c]{@{}l@{}}66.97\\ $\pm$0.73\end{tabular}}          & {\begin{tabular}[c]{@{}l@{}}59.78\\ $\pm$0.32\end{tabular}}          & {\begin{tabular}[c]{@{}l@{}}52.62\\ $\pm$0.76\end{tabular}}          & {\begin{tabular}[c]{@{}l@{}}50.49\\ $\pm$0.51\end{tabular}}          & {\begin{tabular}[c]{@{}l@{}}48.54\\ $\pm$0.35\end{tabular}}          & {\begin{tabular}[c]{@{}l@{}}46.49\\ $\pm$0.46\end{tabular}}          & {\begin{tabular}[c]{@{}l@{}}44.35\\ $\pm$0.48\end{tabular}}          & {\begin{tabular}[c]{@{}l@{}}41.97\\ $\pm$0.49\end{tabular}}          & {\begin{tabular}[c]{@{}l@{}}40.46\\ $\pm$0.53\end{tabular}}          & {\begin{tabular}[c]{@{}l@{}}38.79\\ $\pm$0.55\end{tabular}}          & {\begin{tabular}[c]{@{}l@{}}51.58\\ $\pm$0.47\end{tabular}}          \\ \hline
{ICARL\cite{Rebuffi2017iCaRLIC}}                                                 & {\begin{tabular}[c]{@{}l@{}}75.73\\ $\pm$0.00\end{tabular}}          & {\begin{tabular}[c]{@{}l@{}}0.95\\ $\pm$0.00\end{tabular}}           & {\begin{tabular}[c]{@{}l@{}}0.87\\ $\pm$0.00\end{tabular}}           & {\begin{tabular}[c]{@{}l@{}}0.8\\ $\pm$0.00\end{tabular}}            & {\begin{tabular}[c]{@{}l@{}}0.74\\ $\pm$0.00\end{tabular}}           & {\begin{tabular}[c]{@{}l@{}}0.69\\ $\pm$0.00\end{tabular}}           & {\begin{tabular}[c]{@{}l@{}}0.65\\ $\pm$0.00\end{tabular}}           & {\begin{tabular}[c]{@{}l@{}}0.61\\ $\pm$0.00\end{tabular}}           & {\begin{tabular}[c]{@{}l@{}}0.58\\ $\pm$0.00\end{tabular}}           & {\begin{tabular}[c]{@{}l@{}}0.55\\ $\pm$0.00\end{tabular}}           & {\begin{tabular}[c]{@{}l@{}}0.52\\ $\pm$0.00\end{tabular}}           & {\begin{tabular}[c]{@{}l@{}}7.52\\ $\pm$0.00\end{tabular}}           \\ \hline
{Rebalance\cite{Hou2019LearningAU}}                                             & {\begin{tabular}[c]{@{}l@{}}74.83\\ $\pm$0.00\end{tabular}}          & {\begin{tabular}[c]{@{}l@{}}68.18\\ $\pm$0.00\end{tabular}}          & {\begin{tabular}[c]{@{}l@{}}47.5\\ $\pm$2.95\end{tabular}}           & {\begin{tabular}[c]{@{}l@{}}41.87\\ $\pm$2.41\end{tabular}}          & {\begin{tabular}[c]{@{}l@{}}37.27\\ $\pm$2.07\end{tabular}}          & {\begin{tabular}[c]{@{}l@{}}33.49\\ $\pm$1.67\end{tabular}}          & {\begin{tabular}[c]{@{}l@{}}29.77\\ $\pm$1.51\end{tabular}}          & {\begin{tabular}[c]{@{}l@{}}26.78\\ $\pm$1.76\end{tabular}}          & {\begin{tabular}[c]{@{}l@{}}24.21\\ $\pm$1.76\end{tabular}}          & {\begin{tabular}[c]{@{}l@{}}22.28\\ $\pm$1.52\end{tabular}}          & {\begin{tabular}[c]{@{}l@{}}20.43\\ $\pm$1.48\end{tabular}}          & {\begin{tabular}[c]{@{}l@{}}38.78\\ $\pm$1.56\end{tabular}}          \\ \hline
{\textbf{FLOWER}}                                       & {\textbf{\begin{tabular}[c]{@{}l@{}}79.02\\ $\pm$0.00\end{tabular}}} & {\textbf{\begin{tabular}[c]{@{}l@{}}72.73\\ $\pm$0.18\end{tabular}}} & {\textbf{\begin{tabular}[c]{@{}l@{}}67.29\\ $\pm$0.24\end{tabular}}} & {\textbf{\begin{tabular}[c]{@{}l@{}}62.74\\ $\pm$0.22\end{tabular}}} & {\textbf{\begin{tabular}[c]{@{}l@{}}58.82\\ $\pm$0.31\end{tabular}}} & {\textbf{\begin{tabular}[c]{@{}l@{}}55.43\\ $\pm$0.22\end{tabular}}} & {\textbf{\begin{tabular}[c]{@{}l@{}}52.63\\ $\pm$0.24\end{tabular}}} & {\textbf{\begin{tabular}[c]{@{}l@{}}50.18\\ $\pm$0.27\end{tabular}}} & {\textbf{\begin{tabular}[c]{@{}l@{}}47.77\\ $\pm$0.34\end{tabular}}} & {\textbf{\begin{tabular}[c]{@{}l@{}}46.05\\ $\pm$0.38\end{tabular}}} & {\textbf{\begin{tabular}[c]{@{}l@{}}44.26\\ $\pm$0.43\end{tabular}}} & {\textbf{\begin{tabular}[c]{@{}l@{}}57.90\\ $\pm$0.26\end{tabular}}} \\ \hline
\end{tabular}
\caption{Classification accuracy with 1-shot setting on 100 base classes CUB-2011 dataset. This table is detailed version of table \ref{tab:1shot} in main paper for CUB dataset.}
\label{tab:1shot_cub}
\end{table*}


\section{Complete Numerical Results Experiments with Different Random Seeds}   
Experiments are carried out to validate the robustness of FLOWER under different random numbers. That is, different random seeds are applied using the miniimagenet problem. Table \ref{tab:difference_seeds} reports our numerical results. It is perceived that different random seeds do not vary numerical results significantly while the standard deviations of different runs are also small.  

\begin{table*}[]
\centering
\small
% \begin{tabularx}{1.0\textwidth}{lXXXXXXXXXXXX\fontsize{3}{5}r}
% \begin{tabularx}{1.0\textwidth}{lXXXXXXXXXXXXr}
\begin{tabular}{lccccccccccccc}
\hline
{}                         & \multicolumn{9}{c}{{Session}}     & {}                      \\  \cline{2-10}  
\multirow{-2}{*}{{Seed}} & {1}              & {2}              & {3}              & {4}              & {5}              & {6}              & {7}              & {8}              & {9}              & \multirow{-2}{*}{{Avg}} \\ \hline
{1997}                            & {\begin{tabular}[c]{@{}c@{}}68.83\\ $\pm$0.0\end{tabular}} & {\begin{tabular}[c]{@{}c@{}}63.27\\ $\pm$0.09\end{tabular}} & {\begin{tabular}[c]{@{}c@{}}59.00\\ $\pm$0.16\end{tabular}} & {\begin{tabular}[c]{@{}c@{}}55.61\\ $\pm$0.18\end{tabular}} & {\begin{tabular}[c]{@{}c@{}}52.64\\ $\pm$0.22\end{tabular}} & {\begin{tabular}[c]{@{}c@{}}49.96\\ $\pm$0.20\end{tabular}} & {\begin{tabular}[c]{@{}c@{}}47.56\\ $\pm$0.18\end{tabular}} & {\begin{tabular}[c]{@{}c@{}}45.86\\ $\pm$0.16\end{tabular}} & {\begin{tabular}[c]{@{}c@{}}44.40\\ $\pm$0.21\end{tabular}} & {\begin{tabular}[c]{@{}c@{}}54.13\\ $\pm$0.16\end{tabular}} \\ \hline
{1998}                            & {\begin{tabular}[c]{@{}c@{}}69.00\\ $\pm$0.0\end{tabular}} & {\begin{tabular}[c]{@{}c@{}}63.73\\ $\pm$0.19\end{tabular}} & {\begin{tabular}[c]{@{}c@{}}59.44\\ $\pm$0.25\end{tabular}} & {\begin{tabular}[c]{@{}c@{}}56.11\\ $\pm$0.19\end{tabular}} & {\begin{tabular}[c]{@{}c@{}}53.35\\ $\pm$0.25\end{tabular}} & {\begin{tabular}[c]{@{}c@{}}50.76\\ $\pm$0.37\end{tabular}} & {\begin{tabular}[c]{@{}c@{}}48.12\\ $\pm$0.34\end{tabular}} & {\begin{tabular}[c]{@{}c@{}}46.23\\ $\pm$0.29\end{tabular}} & {\begin{tabular}[c]{@{}c@{}}44.85\\ $\pm$0.27\end{tabular}} & {\begin{tabular}[c]{@{}c@{}}54.62\\ $\pm$0.24\end{tabular}} \\ \hline
{1999}                            & {\begin{tabular}[c]{@{}c@{}}67.93\\ $\pm$0.0\end{tabular}} & {\begin{tabular}[c]{@{}c@{}}62.34\\ $\pm$0.24\end{tabular}} & {\begin{tabular}[c]{@{}c@{}}58.17\\ $\pm$0.29\end{tabular}} & {\begin{tabular}[c]{@{}c@{}}54.86\\ $\pm$0.44\end{tabular}} & {\begin{tabular}[c]{@{}c@{}}52.17\\ $\pm$0.40\end{tabular}} & {\begin{tabular}[c]{@{}c@{}}49.89\\ $\pm$0.50\end{tabular}} & {\begin{tabular}[c]{@{}c@{}}47.36\\ $\pm$0.46\end{tabular}} & {\begin{tabular}[c]{@{}c@{}}45.71\\ $\pm$0.51\end{tabular}} & {\begin{tabular}[c]{@{}c@{}}44.39\\ $\pm$0.38\end{tabular}} & {\begin{tabular}[c]{@{}c@{}}53.65\\ $\pm$0.36\end{tabular}} \\ \hline
{2000}                            & {\begin{tabular}[c]{@{}c@{}}68.12\\ $\pm$0.0\end{tabular}} & {\begin{tabular}[c]{@{}c@{}}62.88\\ $\pm$0.19\end{tabular}} & {\begin{tabular}[c]{@{}c@{}}58.81\\ $\pm$0.30\end{tabular}} & {\begin{tabular}[c]{@{}c@{}}55.32\\ $\pm$0.39\end{tabular}} & {\begin{tabular}[c]{@{}c@{}}52.38\\ $\pm$0.29\end{tabular}} & {\begin{tabular}[c]{@{}c@{}}49.54\\ $\pm$0.20\end{tabular}} & {\begin{tabular}[c]{@{}c@{}}46.93\\ $\pm$0.25\end{tabular}} & {\begin{tabular}[c]{@{}c@{}}45.01\\ $\pm$0.18\end{tabular}} & {\begin{tabular}[c]{@{}c@{}}43.75\\ $\pm$0.31\end{tabular}} & {\begin{tabular}[c]{@{}c@{}}53.64\\ $\pm$0.23\end{tabular}} \\ \hline
{2001}                            & {\begin{tabular}[c]{@{}c@{}}68.37\\ $\pm$0.0\end{tabular}} & {\begin{tabular}[c]{@{}c@{}}63.24\\ $\pm$0.17\end{tabular}} & {\begin{tabular}[c]{@{}c@{}}59.15\\ $\pm$0.12\end{tabular}} & {\begin{tabular}[c]{@{}c@{}}55.85\\ $\pm$0.12\end{tabular}} & {\begin{tabular}[c]{@{}c@{}}53.06\\ $\pm$0.22\end{tabular}} & {\begin{tabular}[c]{@{}c@{}}50.35\\ $\pm$0.19\end{tabular}} & {\begin{tabular}[c]{@{}c@{}}47.69\\ $\pm$0.20\end{tabular}} & {\begin{tabular}[c]{@{}c@{}}45.82\\ $\pm$0.14\end{tabular}} & {\begin{tabular}[c]{@{}c@{}}44.73\\ $\pm$0.20\end{tabular}} & {\begin{tabular}[c]{@{}c@{}}54.25\\ $\pm$0.15\end{tabular}} \\ \hline
    
\end{tabular}
\caption{Classification accuracy on split MiniImagenet dataset (60 base classes) with different random seeds averaged across 5 times runs.}
\label{tab:difference_seeds}
\end{table*}

\end{appendices}
\vfill


\bibliographystyle{IEEEtran}
\bibliography{ref-bibliography}

\end{document}
